# Supplementary material for: Synthesizing Anyone, Anywhere, in Any Pose
Source: arXiv:2304.03164 source file (2023-11-05)
Supplement: Supplementary file 1 [file appendix.tex]

\section{Experimental Details}

All models are trained with Pytorch 1.12 \cite{paszke2019pytorch} on 4 NVIDIA A100-80GB.
FID and \fidC are computed with Torch Fidelity \cite{obukhov2020torchfidelity}.
For qualitative examples, we use multi-modal truncation \cite{Mokady2022} for sampling diverse high quality samples.
\methodName is computationally efficient, where Config E processes $\sim 25$ images per second on an NVIDIA RTX 3090 for single-image inference with unoptimized Pytorch \cite{paszke2019pytorch}.
For computing OKS, we use the \href{https://github.com/ViTAE-Transformer/ViTPose/blob/ec43a105e4a1f3b91ff77ec71a6f49a7501503af/configs/body/2d_kpt_sview_rgb_img/topdown_heatmap/coco/ViTPose_huge_coco_256x192.py}{VITPose-H*} trained on COCO \cite{Lin2014COCO}, AI Challenger, MPII and CrowdPose 

\paragraph{Discriminator Architecture}
We use identical discriminators architectures for the different resolutions.
Each $D_\ell$ (inputting features from the projection $P_\ell$) consists of three convolutions with 512 channels, where the output of $D_\ell$ is half the spatial resolution of $P_\ell$.
We use spectral normalization for each convolution, and each convolution is followed by BatchNorm2d \cite{Ioffe2015} and LeakyReLU \cite{leakyReLU}, except the last.
In total, the discriminator has 5.3M trainable parameters per feature network.
For convolutional feature networks, we upsample the image to $288 \times 160$, whereas for ViT we upsample/downsample to $224 \times 224$.
|

\paragraph{Generator Architecture}
Our generator architecture is similar to the architecture used by \cite{Hukkelas2022a} with the modifications stated in the main paper and the following.
We change the operation order of each convolution to instance normalization $\rightarrow$ style modulation $\rightarrow$ convolution.
We use exponential moving average (EMA) \cite{Yazc2018} for the generator parameters with a warmup period following \cite{Karras2019b}.

\paragraph{Training Hyperparameters}
Experimental hyperparameters are given in \Cref{tab:hyperparameters}.

\begin{table*}[t]
    \caption{
        Training hyperparameters.
        \textbf{*} Batch size/channel size is given per resolution, where "18" refers to the resolution $18 \times 10$.
        $\dagger$ Decoder is symmetric.
        }
    \label{tab:hyperparameters}
    \centering
    \begin{adjustbox}{max width=\linewidth}
    \begin{tabular}{lcc}
        \hline
        & Config A-D & Config E \\
        \hline
        Adam parameters & lr=0.002, $\beta_1=0.0, \beta_2=0.099$ & Same\\
        GPUs & 4x A100-80GB & 8x A100-80GB \\
        Batch size* & 18: 512, 36: 512, 72: 512 & 18: 1024, 36: 1024, 72: 1024, 144: 512, 288: 128 \\
        EMA & 0.9976 & Same \\
        Discriminator trainable parameters & 5.3M per feature network & Same \\
        Data Augmentation & Horizontal flip & Same \\
        Number of images seen by the discriminator & 50M each resolution & 18: 300M, 36: 200M, 72: 160M, 144: 110M, 288: 110M\\
        \hline
        Generator parameters ($72\times 40$) (Config A-D) & 62.2M & 110.4M\\
        Generator parameters ($288\times 160$)  &  Not trained & 124.2M\\
        Convolution Channels* & 18: 512, 36: 512, 72: 512, 144: 256, 288: 128 & Same \\
        Number of residual blocks per generator encoder block $\dagger$ & 1 & 2 \\

        \hline
    \end{tabular}
    \end{adjustbox}

\end{table*}

\section{Cleaning the FDH Dataset}
We clean the FDH dataset by refining the keypoint annotations with the top-down pose estimation model VITPose \cite{Xu22VITPose}
\footnote{We use the \href{https://github.com/ViTAE-Transformer/ViTPose/blob/ec43a105e4a1f3b91ff77ec71a6f49a7501503af/configs/body/2d_kpt_sview_rgb_img/topdown_heatmap/coco/ViTPose_huge_coco_256x192.py}{VITPose-H*} trained on COCO \cite{Lin2014COCO}, AI Challenger, MPII and CrowdPose }.
VITPose \cite{Xu22VITPose} estimates 17 keypoints following the COCO \cite{Lin2014COCO} format given the image from the FDH dataset and the minimal enclosing bounding box of the embedding mask (named E\_mask in the FDH dataset).
Given the original keypoints and the new keypoints from VITPose, we select one of them given how well the annotation matches the DensePose annotation (from CSE \cite{Neverova2020}) in the FDH dataset.
Specifically, by using pixel-to-vertex correspondences we segment each surface pixel into a semantic body part \footnote{We use an open source semantic segmentation of the SMPL model, found \href{https://raw.githubusercontent.com/Meshcapade/wiki/main/assets/SMPL_body_segmentation/smpl/smpl_vert_segmentation.json}{here}.}.
Then, we count the number of keypoints matches to the correct body part (e.g. the keypoint "eye" should match to the body part "head").
The annotation with the highest percentage correct matches is selected.
From this selection, 19,722 of 30K images  are updated for the validation dataset, and 1,199,927 out of 1,829,496 images in the training dataset are updated.

\section{Qualitative Examples of Different Discriminator Feature Networks}
The generated images are given in \Cref{fig:generated_images_different_fnets}.
\begin{figure*}
    \centering
    \begin{subfigure}{0.24\textwidth}
        \includegraphics[width=\textwidth]{appendix_figures/image_dump_square4/im72_rn50_IN_MAD.png}
        \caption*{ImageNet - RN50}
    \end{subfigure}
    \begin{subfigure}{0.24\textwidth}
        \includegraphics[width=\textwidth]{appendix_figures/image_dump_square4/im72_rn50_CSE_MAD.png}
        \caption*{CSE - RN50}
    \end{subfigure}
    \begin{subfigure}{0.24\textwidth}
        \includegraphics[width=\textwidth]{appendix_figures/image_dump_square4/im72_CLIP_MAD.png}
        \caption*{CLIP - RN50}
    \end{subfigure}
    \begin{subfigure}{0.24\textwidth}
        \hfill
    \end{subfigure}
    \hfill
    \begin{subfigure}{0.24\textwidth}
        \includegraphics[width=\textwidth]{appendix_figures/image_dump_square4/im72_VIT_IN_MAD.png}
        \caption*{ImageNet - ViT-B16}
    \end{subfigure}
    \begin{subfigure}{0.24\textwidth}
            \hfill
        \end{subfigure}
    \begin{subfigure}{0.24\textwidth}%
        \includegraphics[width=\textwidth]{appendix_figures/image_dump_square4/im72_VIT_CLIP_MAD.png}
        \caption*{CLIP - ViT-B16}
    \end{subfigure}
    \begin{subfigure}{0.24\textwidth}
        \includegraphics[width=\textwidth]{appendix_figures/image_dump_square4/im72_MAE_MAD.png}
        \caption*{MAE - ViT-B16}
    \end{subfigure}
    \begin{subfigure}{0.24\textwidth}
        \includegraphics[width=\textwidth]{appendix_figures/image_dump_square4/im72_effnet_MAD.png}
        \caption*{ImageNet - EfficientNet-Lite0}
    \end{subfigure}
    \begin{subfigure}{0.24\textwidth}
        \includegraphics[width=\textwidth]{appendix_figures/image_dump_square4/im72_MAD.png}
        \caption*{ViT-B16$_\text{MAE}$ + RN50$_\text{CLIP}$}
    \end{subfigure}
    \begin{subfigure}{0.24\textwidth}
        \includegraphics[width=\textwidth]{appendix_figures/image_dump_square4/im72_MAEL_clip_MAD.png}
        \caption*{ViT-L16$_\text{MAE}$ + RN50$_\text{CLIP}$}
    \end{subfigure}
    \begin{subfigure}{0.24\textwidth}
        \includegraphics[width=\textwidth]{appendix_figures/image_dump_square4/im72_MAEL_MAD.png}
        \caption*{ViT-L16$_\text{MAE}$}
    \end{subfigure}
    \caption{
        Generated images with Config B using different feature networks stated below each image.
        Images are given in full resolution ($72 \times 40$), and we recommend the reader to zoom in.
        }
    \label{fig:generated_images_different_fnets}

\end{figure*}

\section{Random Generated Examples and Comparison Surface-Guided GANs}
Randomly selected images comparing \methodName to SG-GAN \cite{Hukkelas2022a} are given in the following figures:
\Cref{fig:fdh_random0},
\ref{fig:fdh_random1},
\ref{fig:fdh_random2},
\ref{fig:fdh_random3},
\ref{fig:fdh_random4},
\ref{fig:fdh_random5},
\ref{fig:fdh_random6},
\ref{fig:fdh_random8},
\ref{fig:fdh_random9},
\ref{fig:fdh_random10},
\ref{fig:fdh_random11},
\ref{fig:fdh_random12},
\ref{fig:fdh_random13},
\ref{fig:fdh_random14},
\ref{fig:fdh_random15},
\ref{fig:fdh_random16}, and
\ref{fig:fdh_random17}.

\begin{figure*}[t]
\centering
\begin{subfigure}[t]{0.125\textwidth}
\includegraphics[width=\textwidth]{appendix_figures/random_FDH/styleganL/singles/10200/original.png}
\includegraphics[width=\textwidth]{appendix_figures/random_FDH/styleganL/singles/10327/original.png}
\includegraphics[width=\textwidth]{appendix_figures/random_FDH/styleganL/singles/10368/original.png}
\includegraphics[width=\textwidth]{appendix_figures/random_FDH/styleganL/singles/10799/original.png}
\includegraphics[width=\textwidth]{appendix_figures/random_FDH/styleganL/singles/11122/original.png}
\caption{Original}
\end{subfigure}%%
\begin{subfigure}[t]{0.125\textwidth}
\includegraphics[width=\textwidth]{appendix_figures/random_FDH/styleganL/singles/10200/masked_keypoints.png}
\includegraphics[width=\textwidth]{appendix_figures/random_FDH/styleganL/singles/10327/masked_keypoints.png}
\includegraphics[width=\textwidth]{appendix_figures/random_FDH/styleganL/singles/10368/masked_keypoints.png}
\includegraphics[width=\textwidth]{appendix_figures/random_FDH/styleganL/singles/10799/masked_keypoints.png}
\includegraphics[width=\textwidth]{appendix_figures/random_FDH/styleganL/singles/11122/masked_keypoints.png}
\caption{Condition}
\end{subfigure}%%
\begin{subfigure}[t]{0.125\textwidth}
\includegraphics[width=\textwidth]{appendix_figures/random_FDH/styleganL/singles/10200/fakes/0.png}
\includegraphics[width=\textwidth]{appendix_figures/random_FDH/styleganL/singles/10327/fakes/0.png}
\includegraphics[width=\textwidth]{appendix_figures/random_FDH/styleganL/singles/10368/fakes/0.png}
\includegraphics[width=\textwidth]{appendix_figures/random_FDH/styleganL/singles/10799/fakes/0.png}
\includegraphics[width=\textwidth]{appendix_figures/random_FDH/styleganL/singles/11122/fakes/0.png}
\caption{SG-GAN}
\end{subfigure}%%
\begin{subfigure}[t]{0.125\textwidth}
\includegraphics[width=\textwidth]{appendix_figures/random_FDH/styleganL/singles/10200/fakes/1.png}
\includegraphics[width=\textwidth]{appendix_figures/random_FDH/styleganL/singles/10327/fakes/1.png}
\includegraphics[width=\textwidth]{appendix_figures/random_FDH/styleganL/singles/10368/fakes/1.png}
\includegraphics[width=\textwidth]{appendix_figures/random_FDH/styleganL/singles/10799/fakes/1.png}
\includegraphics[width=\textwidth]{appendix_figures/random_FDH/styleganL/singles/11122/fakes/1.png}
\caption{SG-GAN}
\end{subfigure}%%
\begin{subfigure}[t]{0.125\textwidth}
\includegraphics[width=\textwidth]{appendix_figures/random_FDH/styleganL/singles/10200/fakes/2.png}
\includegraphics[width=\textwidth]{appendix_figures/random_FDH/styleganL/singles/10327/fakes/2.png}
\includegraphics[width=\textwidth]{appendix_figures/random_FDH/styleganL/singles/10368/fakes/2.png}
\includegraphics[width=\textwidth]{appendix_figures/random_FDH/styleganL/singles/10799/fakes/2.png}
\includegraphics[width=\textwidth]{appendix_figures/random_FDH/styleganL/singles/11122/fakes/2.png}
\caption{SG-GAN}
\end{subfigure}%%
\begin{subfigure}[t]{0.125\textwidth}
\includegraphics[width=\textwidth]{appendix_figures/random_FDH/im288/singles/10200/fakes/0.png}
\includegraphics[width=\textwidth]{appendix_figures/random_FDH/im288/singles/10327/fakes/0.png}
\includegraphics[width=\textwidth]{appendix_figures/random_FDH/im288/singles/10368/fakes/0.png}
\includegraphics[width=\textwidth]{appendix_figures/random_FDH/im288/singles/10799/fakes/0.png}
\includegraphics[width=\textwidth]{appendix_figures/random_FDH/im288/singles/11122/fakes/0.png}
\caption{\methodName}
\end{subfigure}%%
\begin{subfigure}[t]{0.125\textwidth}
\includegraphics[width=\textwidth]{appendix_figures/random_FDH/im288/singles/10200/fakes/1.png}
\includegraphics[width=\textwidth]{appendix_figures/random_FDH/im288/singles/10327/fakes/1.png}
\includegraphics[width=\textwidth]{appendix_figures/random_FDH/im288/singles/10368/fakes/1.png}
\includegraphics[width=\textwidth]{appendix_figures/random_FDH/im288/singles/10799/fakes/1.png}
\includegraphics[width=\textwidth]{appendix_figures/random_FDH/im288/singles/11122/fakes/1.png}
\caption{\methodName}
\end{subfigure}%%
\begin{subfigure}[t]{0.125\textwidth}
\includegraphics[width=\textwidth]{appendix_figures/random_FDH/im288/singles/10200/fakes/2.png}
\includegraphics[width=\textwidth]{appendix_figures/random_FDH/im288/singles/10327/fakes/2.png}
\includegraphics[width=\textwidth]{appendix_figures/random_FDH/im288/singles/10368/fakes/2.png}
\includegraphics[width=\textwidth]{appendix_figures/random_FDH/im288/singles/10799/fakes/2.png}
\includegraphics[width=\textwidth]{appendix_figures/random_FDH/im288/singles/11122/fakes/2.png}
\caption{\methodName}
\end{subfigure}%%
\caption{Random generated examples from FDH \cite{Hukkelas2022a} comparing \methodName to SG-GAN \cite{Hukkelas2022a}.
Note that all examples are generated with multi-modal truncation.
Surface map is not used by \methodName.}
\label{fig:fdh_random0}
\end{figure*}
\begin{figure*}[t]
\centering
\begin{subfigure}[t]{0.125\textwidth}
\includegraphics[width=\textwidth]{appendix_figures/random_FDH/styleganL/singles/11723/original.png}
\includegraphics[width=\textwidth]{appendix_figures/random_FDH/styleganL/singles/12134/original.png}
\includegraphics[width=\textwidth]{appendix_figures/random_FDH/styleganL/singles/12372/original.png}
\includegraphics[width=\textwidth]{appendix_figures/random_FDH/styleganL/singles/12676/original.png}
\includegraphics[width=\textwidth]{appendix_figures/random_FDH/styleganL/singles/13062/original.png}
\caption{Original}
\end{subfigure}%%
\begin{subfigure}[t]{0.125\textwidth}
\includegraphics[width=\textwidth]{appendix_figures/random_FDH/styleganL/singles/11723/masked_keypoints.png}
\includegraphics[width=\textwidth]{appendix_figures/random_FDH/styleganL/singles/12134/masked_keypoints.png}
\includegraphics[width=\textwidth]{appendix_figures/random_FDH/styleganL/singles/12372/masked_keypoints.png}
\includegraphics[width=\textwidth]{appendix_figures/random_FDH/styleganL/singles/12676/masked_keypoints.png}
\includegraphics[width=\textwidth]{appendix_figures/random_FDH/styleganL/singles/13062/masked_keypoints.png}
\caption{Condition}
\end{subfigure}%%
\begin{subfigure}[t]{0.125\textwidth}
\includegraphics[width=\textwidth]{appendix_figures/random_FDH/styleganL/singles/11723/fakes/0.png}
\includegraphics[width=\textwidth]{appendix_figures/random_FDH/styleganL/singles/12134/fakes/0.png}
\includegraphics[width=\textwidth]{appendix_figures/random_FDH/styleganL/singles/12372/fakes/0.png}
\includegraphics[width=\textwidth]{appendix_figures/random_FDH/styleganL/singles/12676/fakes/0.png}
\includegraphics[width=\textwidth]{appendix_figures/random_FDH/styleganL/singles/13062/fakes/0.png}
\caption{SG-GAN}
\end{subfigure}%%
\begin{subfigure}[t]{0.125\textwidth}
\includegraphics[width=\textwidth]{appendix_figures/random_FDH/styleganL/singles/11723/fakes/1.png}
\includegraphics[width=\textwidth]{appendix_figures/random_FDH/styleganL/singles/12134/fakes/1.png}
\includegraphics[width=\textwidth]{appendix_figures/random_FDH/styleganL/singles/12372/fakes/1.png}
\includegraphics[width=\textwidth]{appendix_figures/random_FDH/styleganL/singles/12676/fakes/1.png}
\includegraphics[width=\textwidth]{appendix_figures/random_FDH/styleganL/singles/13062/fakes/1.png}
\caption{SG-GAN}
\end{subfigure}%%
\begin{subfigure}[t]{0.125\textwidth}
\includegraphics[width=\textwidth]{appendix_figures/random_FDH/styleganL/singles/11723/fakes/2.png}
\includegraphics[width=\textwidth]{appendix_figures/random_FDH/styleganL/singles/12134/fakes/2.png}
\includegraphics[width=\textwidth]{appendix_figures/random_FDH/styleganL/singles/12372/fakes/2.png}
\includegraphics[width=\textwidth]{appendix_figures/random_FDH/styleganL/singles/12676/fakes/2.png}
\includegraphics[width=\textwidth]{appendix_figures/random_FDH/styleganL/singles/13062/fakes/2.png}
\caption{SG-GAN}
\end{subfigure}%%
\begin{subfigure}[t]{0.125\textwidth}
\includegraphics[width=\textwidth]{appendix_figures/random_FDH/im288/singles/11723/fakes/0.png}
\includegraphics[width=\textwidth]{appendix_figures/random_FDH/im288/singles/12134/fakes/0.png}
\includegraphics[width=\textwidth]{appendix_figures/random_FDH/im288/singles/12372/fakes/0.png}
\includegraphics[width=\textwidth]{appendix_figures/random_FDH/im288/singles/12676/fakes/0.png}
\includegraphics[width=\textwidth]{appendix_figures/random_FDH/im288/singles/13062/fakes/0.png}
\caption{\methodName}
\end{subfigure}%%
\begin{subfigure}[t]{0.125\textwidth}
\includegraphics[width=\textwidth]{appendix_figures/random_FDH/im288/singles/11723/fakes/1.png}
\includegraphics[width=\textwidth]{appendix_figures/random_FDH/im288/singles/12134/fakes/1.png}
\includegraphics[width=\textwidth]{appendix_figures/random_FDH/im288/singles/12372/fakes/1.png}
\includegraphics[width=\textwidth]{appendix_figures/random_FDH/im288/singles/12676/fakes/1.png}
\includegraphics[width=\textwidth]{appendix_figures/random_FDH/im288/singles/13062/fakes/1.png}
\caption{\methodName}
\end{subfigure}%%
\begin{subfigure}[t]{0.125\textwidth}
\includegraphics[width=\textwidth]{appendix_figures/random_FDH/im288/singles/11723/fakes/2.png}
\includegraphics[width=\textwidth]{appendix_figures/random_FDH/im288/singles/12134/fakes/2.png}
\includegraphics[width=\textwidth]{appendix_figures/random_FDH/im288/singles/12372/fakes/2.png}
\includegraphics[width=\textwidth]{appendix_figures/random_FDH/im288/singles/12676/fakes/2.png}
\includegraphics[width=\textwidth]{appendix_figures/random_FDH/im288/singles/13062/fakes/2.png}
\caption{\methodName}
\end{subfigure}%%
\caption{Random generated examples from FDH \cite{Hukkelas2022a} comparing \methodName to SG-GAN \cite{Hukkelas2022a}.
Note that all examples are generated with multi-modal truncation.
Surface map is not used by \methodName.}
\label{fig:fdh_random1}
\end{figure*}
\begin{figure*}[t]
\centering
\begin{subfigure}[t]{0.125\textwidth}
\includegraphics[width=\textwidth]{appendix_figures/random_FDH/styleganL/singles/13123/original.png}
\includegraphics[width=\textwidth]{appendix_figures/random_FDH/styleganL/singles/13754/original.png}
\includegraphics[width=\textwidth]{appendix_figures/random_FDH/styleganL/singles/14116/original.png}
\includegraphics[width=\textwidth]{appendix_figures/random_FDH/styleganL/singles/14627/original.png}
\includegraphics[width=\textwidth]{appendix_figures/random_FDH/styleganL/singles/14650/original.png}
\caption{Original}
\end{subfigure}%%
\begin{subfigure}[t]{0.125\textwidth}
\includegraphics[width=\textwidth]{appendix_figures/random_FDH/styleganL/singles/13123/masked_keypoints.png}
\includegraphics[width=\textwidth]{appendix_figures/random_FDH/styleganL/singles/13754/masked_keypoints.png}
\includegraphics[width=\textwidth]{appendix_figures/random_FDH/styleganL/singles/14116/masked_keypoints.png}
\includegraphics[width=\textwidth]{appendix_figures/random_FDH/styleganL/singles/14627/masked_keypoints.png}
\includegraphics[width=\textwidth]{appendix_figures/random_FDH/styleganL/singles/14650/masked_keypoints.png}
\caption{Condition}
\end{subfigure}%%
\begin{subfigure}[t]{0.125\textwidth}
\includegraphics[width=\textwidth]{appendix_figures/random_FDH/styleganL/singles/13123/fakes/0.png}
\includegraphics[width=\textwidth]{appendix_figures/random_FDH/styleganL/singles/13754/fakes/0.png}
\includegraphics[width=\textwidth]{appendix_figures/random_FDH/styleganL/singles/14116/fakes/0.png}
\includegraphics[width=\textwidth]{appendix_figures/random_FDH/styleganL/singles/14627/fakes/0.png}
\includegraphics[width=\textwidth]{appendix_figures/random_FDH/styleganL/singles/14650/fakes/0.png}
\caption{SG-GAN}
\end{subfigure}%%
\begin{subfigure}[t]{0.125\textwidth}
\includegraphics[width=\textwidth]{appendix_figures/random_FDH/styleganL/singles/13123/fakes/1.png}
\includegraphics[width=\textwidth]{appendix_figures/random_FDH/styleganL/singles/13754/fakes/1.png}
\includegraphics[width=\textwidth]{appendix_figures/random_FDH/styleganL/singles/14116/fakes/1.png}
\includegraphics[width=\textwidth]{appendix_figures/random_FDH/styleganL/singles/14627/fakes/1.png}
\includegraphics[width=\textwidth]{appendix_figures/random_FDH/styleganL/singles/14650/fakes/1.png}
\caption{SG-GAN}
\end{subfigure}%%
\begin{subfigure}[t]{0.125\textwidth}
\includegraphics[width=\textwidth]{appendix_figures/random_FDH/styleganL/singles/13123/fakes/2.png}
\includegraphics[width=\textwidth]{appendix_figures/random_FDH/styleganL/singles/13754/fakes/2.png}
\includegraphics[width=\textwidth]{appendix_figures/random_FDH/styleganL/singles/14116/fakes/2.png}
\includegraphics[width=\textwidth]{appendix_figures/random_FDH/styleganL/singles/14627/fakes/2.png}
\includegraphics[width=\textwidth]{appendix_figures/random_FDH/styleganL/singles/14650/fakes/2.png}
\caption{SG-GAN}
\end{subfigure}%%
\begin{subfigure}[t]{0.125\textwidth}
\includegraphics[width=\textwidth]{appendix_figures/random_FDH/im288/singles/13123/fakes/0.png}
\includegraphics[width=\textwidth]{appendix_figures/random_FDH/im288/singles/13754/fakes/0.png}
\includegraphics[width=\textwidth]{appendix_figures/random_FDH/im288/singles/14116/fakes/0.png}
\includegraphics[width=\textwidth]{appendix_figures/random_FDH/im288/singles/14627/fakes/0.png}
\includegraphics[width=\textwidth]{appendix_figures/random_FDH/im288/singles/14650/fakes/0.png}
\caption{\methodName}
\end{subfigure}%%
\begin{subfigure}[t]{0.125\textwidth}
\includegraphics[width=\textwidth]{appendix_figures/random_FDH/im288/singles/13123/fakes/1.png}
\includegraphics[width=\textwidth]{appendix_figures/random_FDH/im288/singles/13754/fakes/1.png}
\includegraphics[width=\textwidth]{appendix_figures/random_FDH/im288/singles/14116/fakes/1.png}
\includegraphics[width=\textwidth]{appendix_figures/random_FDH/im288/singles/14627/fakes/1.png}
\includegraphics[width=\textwidth]{appendix_figures/random_FDH/im288/singles/14650/fakes/1.png}
\caption{\methodName}
\end{subfigure}%%
\begin{subfigure}[t]{0.125\textwidth}
\includegraphics[width=\textwidth]{appendix_figures/random_FDH/im288/singles/13123/fakes/2.png}
\includegraphics[width=\textwidth]{appendix_figures/random_FDH/im288/singles/13754/fakes/2.png}
\includegraphics[width=\textwidth]{appendix_figures/random_FDH/im288/singles/14116/fakes/2.png}
\includegraphics[width=\textwidth]{appendix_figures/random_FDH/im288/singles/14627/fakes/2.png}
\includegraphics[width=\textwidth]{appendix_figures/random_FDH/im288/singles/14650/fakes/2.png}
\caption{\methodName}
\end{subfigure}%%
\caption{Random generated examples from FDH \cite{Hukkelas2022a} comparing \methodName to SG-GAN \cite{Hukkelas2022a}.
Note that all examples are generated with multi-modal truncation.
Surface map is not used by \methodName.}
\label{fig:fdh_random2}
\end{figure*}
\begin{figure*}[t]
\centering
\begin{subfigure}[t]{0.125\textwidth}
\includegraphics[width=\textwidth]{appendix_figures/random_FDH/styleganL/singles/14879/original.png}
\includegraphics[width=\textwidth]{appendix_figures/random_FDH/styleganL/singles/14935/original.png}
\includegraphics[width=\textwidth]{appendix_figures/random_FDH/styleganL/singles/15115/original.png}
\includegraphics[width=\textwidth]{appendix_figures/random_FDH/styleganL/singles/15186/original.png}
\includegraphics[width=\textwidth]{appendix_figures/random_FDH/styleganL/singles/15246/original.png}
\caption{Original}
\end{subfigure}%%
\begin{subfigure}[t]{0.125\textwidth}
\includegraphics[width=\textwidth]{appendix_figures/random_FDH/styleganL/singles/14879/masked_keypoints.png}
\includegraphics[width=\textwidth]{appendix_figures/random_FDH/styleganL/singles/14935/masked_keypoints.png}
\includegraphics[width=\textwidth]{appendix_figures/random_FDH/styleganL/singles/15115/masked_keypoints.png}
\includegraphics[width=\textwidth]{appendix_figures/random_FDH/styleganL/singles/15186/masked_keypoints.png}
\includegraphics[width=\textwidth]{appendix_figures/random_FDH/styleganL/singles/15246/masked_keypoints.png}
\caption{Condition}
\end{subfigure}%%
\begin{subfigure}[t]{0.125\textwidth}
\includegraphics[width=\textwidth]{appendix_figures/random_FDH/styleganL/singles/14879/fakes/0.png}
\includegraphics[width=\textwidth]{appendix_figures/random_FDH/styleganL/singles/14935/fakes/0.png}
\includegraphics[width=\textwidth]{appendix_figures/random_FDH/styleganL/singles/15115/fakes/0.png}
\includegraphics[width=\textwidth]{appendix_figures/random_FDH/styleganL/singles/15186/fakes/0.png}
\includegraphics[width=\textwidth]{appendix_figures/random_FDH/styleganL/singles/15246/fakes/0.png}
\caption{SG-GAN}
\end{subfigure}%%
\begin{subfigure}[t]{0.125\textwidth}
\includegraphics[width=\textwidth]{appendix_figures/random_FDH/styleganL/singles/14879/fakes/1.png}
\includegraphics[width=\textwidth]{appendix_figures/random_FDH/styleganL/singles/14935/fakes/1.png}
\includegraphics[width=\textwidth]{appendix_figures/random_FDH/styleganL/singles/15115/fakes/1.png}
\includegraphics[width=\textwidth]{appendix_figures/random_FDH/styleganL/singles/15186/fakes/1.png}
\includegraphics[width=\textwidth]{appendix_figures/random_FDH/styleganL/singles/15246/fakes/1.png}
\caption{SG-GAN}
\end{subfigure}%%
\begin{subfigure}[t]{0.125\textwidth}
\includegraphics[width=\textwidth]{appendix_figures/random_FDH/styleganL/singles/14879/fakes/2.png}
\includegraphics[width=\textwidth]{appendix_figures/random_FDH/styleganL/singles/14935/fakes/2.png}
\includegraphics[width=\textwidth]{appendix_figures/random_FDH/styleganL/singles/15115/fakes/2.png}
\includegraphics[width=\textwidth]{appendix_figures/random_FDH/styleganL/singles/15186/fakes/2.png}
\includegraphics[width=\textwidth]{appendix_figures/random_FDH/styleganL/singles/15246/fakes/2.png}
\caption{SG-GAN}
\end{subfigure}%%
\begin{subfigure}[t]{0.125\textwidth}
\includegraphics[width=\textwidth]{appendix_figures/random_FDH/im288/singles/14879/fakes/0.png}
\includegraphics[width=\textwidth]{appendix_figures/random_FDH/im288/singles/14935/fakes/0.png}
\includegraphics[width=\textwidth]{appendix_figures/random_FDH/im288/singles/15115/fakes/0.png}
\includegraphics[width=\textwidth]{appendix_figures/random_FDH/im288/singles/15186/fakes/0.png}
\includegraphics[width=\textwidth]{appendix_figures/random_FDH/im288/singles/15246/fakes/0.png}
\caption{\methodName}
\end{subfigure}%%
\begin{subfigure}[t]{0.125\textwidth}
\includegraphics[width=\textwidth]{appendix_figures/random_FDH/im288/singles/14879/fakes/1.png}
\includegraphics[width=\textwidth]{appendix_figures/random_FDH/im288/singles/14935/fakes/1.png}
\includegraphics[width=\textwidth]{appendix_figures/random_FDH/im288/singles/15115/fakes/1.png}
\includegraphics[width=\textwidth]{appendix_figures/random_FDH/im288/singles/15186/fakes/1.png}
\includegraphics[width=\textwidth]{appendix_figures/random_FDH/im288/singles/15246/fakes/1.png}
\caption{\methodName}
\end{subfigure}%%
\begin{subfigure}[t]{0.125\textwidth}
\includegraphics[width=\textwidth]{appendix_figures/random_FDH/im288/singles/14879/fakes/2.png}
\includegraphics[width=\textwidth]{appendix_figures/random_FDH/im288/singles/14935/fakes/2.png}
\includegraphics[width=\textwidth]{appendix_figures/random_FDH/im288/singles/15115/fakes/2.png}
\includegraphics[width=\textwidth]{appendix_figures/random_FDH/im288/singles/15186/fakes/2.png}
\includegraphics[width=\textwidth]{appendix_figures/random_FDH/im288/singles/15246/fakes/2.png}
\caption{\methodName}
\end{subfigure}%%
\caption{Random generated examples from FDH \cite{Hukkelas2022a} comparing \methodName to SG-GAN \cite{Hukkelas2022a}.
Note that all examples are generated with multi-modal truncation.
Surface map is not used by \methodName.}
\label{fig:fdh_random3}
\end{figure*}
\begin{figure*}[t]
\centering
\begin{subfigure}[t]{0.125\textwidth}
\includegraphics[width=\textwidth]{appendix_figures/random_FDH/styleganL/singles/15430/original.png}
\includegraphics[width=\textwidth]{appendix_figures/random_FDH/styleganL/singles/15832/original.png}
\includegraphics[width=\textwidth]{appendix_figures/random_FDH/styleganL/singles/16298/original.png}
\includegraphics[width=\textwidth]{appendix_figures/random_FDH/styleganL/singles/16321/original.png}
\includegraphics[width=\textwidth]{appendix_figures/random_FDH/styleganL/singles/16921/original.png}
\caption{Original}
\end{subfigure}%%
\begin{subfigure}[t]{0.125\textwidth}
\includegraphics[width=\textwidth]{appendix_figures/random_FDH/styleganL/singles/15430/masked_keypoints.png}
\includegraphics[width=\textwidth]{appendix_figures/random_FDH/styleganL/singles/15832/masked_keypoints.png}
\includegraphics[width=\textwidth]{appendix_figures/random_FDH/styleganL/singles/16298/masked_keypoints.png}
\includegraphics[width=\textwidth]{appendix_figures/random_FDH/styleganL/singles/16321/masked_keypoints.png}
\includegraphics[width=\textwidth]{appendix_figures/random_FDH/styleganL/singles/16921/masked_keypoints.png}
\caption{Condition}
\end{subfigure}%%
\begin{subfigure}[t]{0.125\textwidth}
\includegraphics[width=\textwidth]{appendix_figures/random_FDH/styleganL/singles/15430/fakes/0.png}
\includegraphics[width=\textwidth]{appendix_figures/random_FDH/styleganL/singles/15832/fakes/0.png}
\includegraphics[width=\textwidth]{appendix_figures/random_FDH/styleganL/singles/16298/fakes/0.png}
\includegraphics[width=\textwidth]{appendix_figures/random_FDH/styleganL/singles/16321/fakes/0.png}
\includegraphics[width=\textwidth]{appendix_figures/random_FDH/styleganL/singles/16921/fakes/0.png}
\caption{SG-GAN}
\end{subfigure}%%
\begin{subfigure}[t]{0.125\textwidth}
\includegraphics[width=\textwidth]{appendix_figures/random_FDH/styleganL/singles/15430/fakes/1.png}
\includegraphics[width=\textwidth]{appendix_figures/random_FDH/styleganL/singles/15832/fakes/1.png}
\includegraphics[width=\textwidth]{appendix_figures/random_FDH/styleganL/singles/16298/fakes/1.png}
\includegraphics[width=\textwidth]{appendix_figures/random_FDH/styleganL/singles/16321/fakes/1.png}
\includegraphics[width=\textwidth]{appendix_figures/random_FDH/styleganL/singles/16921/fakes/1.png}
\caption{SG-GAN}
\end{subfigure}%%
\begin{subfigure}[t]{0.125\textwidth}
\includegraphics[width=\textwidth]{appendix_figures/random_FDH/styleganL/singles/15430/fakes/2.png}
\includegraphics[width=\textwidth]{appendix_figures/random_FDH/styleganL/singles/15832/fakes/2.png}
\includegraphics[width=\textwidth]{appendix_figures/random_FDH/styleganL/singles/16298/fakes/2.png}
\includegraphics[width=\textwidth]{appendix_figures/random_FDH/styleganL/singles/16321/fakes/2.png}
\includegraphics[width=\textwidth]{appendix_figures/random_FDH/styleganL/singles/16921/fakes/2.png}
\caption{SG-GAN}
\end{subfigure}%%
\begin{subfigure}[t]{0.125\textwidth}
\includegraphics[width=\textwidth]{appendix_figures/random_FDH/im288/singles/15430/fakes/0.png}
\includegraphics[width=\textwidth]{appendix_figures/random_FDH/im288/singles/15832/fakes/0.png}
\includegraphics[width=\textwidth]{appendix_figures/random_FDH/im288/singles/16298/fakes/0.png}
\includegraphics[width=\textwidth]{appendix_figures/random_FDH/im288/singles/16321/fakes/0.png}
\includegraphics[width=\textwidth]{appendix_figures/random_FDH/im288/singles/16921/fakes/0.png}
\caption{\methodName}
\end{subfigure}%%
\begin{subfigure}[t]{0.125\textwidth}
\includegraphics[width=\textwidth]{appendix_figures/random_FDH/im288/singles/15430/fakes/1.png}
\includegraphics[width=\textwidth]{appendix_figures/random_FDH/im288/singles/15832/fakes/1.png}
\includegraphics[width=\textwidth]{appendix_figures/random_FDH/im288/singles/16298/fakes/1.png}
\includegraphics[width=\textwidth]{appendix_figures/random_FDH/im288/singles/16321/fakes/1.png}
\includegraphics[width=\textwidth]{appendix_figures/random_FDH/im288/singles/16921/fakes/1.png}
\caption{\methodName}
\end{subfigure}%%
\begin{subfigure}[t]{0.125\textwidth}
\includegraphics[width=\textwidth]{appendix_figures/random_FDH/im288/singles/15430/fakes/2.png}
\includegraphics[width=\textwidth]{appendix_figures/random_FDH/im288/singles/15832/fakes/2.png}
\includegraphics[width=\textwidth]{appendix_figures/random_FDH/im288/singles/16298/fakes/2.png}
\includegraphics[width=\textwidth]{appendix_figures/random_FDH/im288/singles/16321/fakes/2.png}
\includegraphics[width=\textwidth]{appendix_figures/random_FDH/im288/singles/16921/fakes/2.png}
\caption{\methodName}
\end{subfigure}%%
\caption{Random generated examples from FDH \cite{Hukkelas2022a} comparing \methodName to SG-GAN \cite{Hukkelas2022a}.
Note that all examples are generated with multi-modal truncation.
Surface map is not used by \methodName.}
\label{fig:fdh_random4}
\end{figure*}
\begin{figure*}[t]
\centering
\begin{subfigure}[t]{0.125\textwidth}
\includegraphics[width=\textwidth]{appendix_figures/random_FDH/styleganL/singles/17043/original.png}
\includegraphics[width=\textwidth]{appendix_figures/random_FDH/styleganL/singles/17089/original.png}
\includegraphics[width=\textwidth]{appendix_figures/random_FDH/styleganL/singles/17098/original.png}
\includegraphics[width=\textwidth]{appendix_figures/random_FDH/styleganL/singles/17455/original.png}
\includegraphics[width=\textwidth]{appendix_figures/random_FDH/styleganL/singles/17591/original.png}
\caption{Original}
\end{subfigure}%%
\begin{subfigure}[t]{0.125\textwidth}
\includegraphics[width=\textwidth]{appendix_figures/random_FDH/styleganL/singles/17043/masked_keypoints.png}
\includegraphics[width=\textwidth]{appendix_figures/random_FDH/styleganL/singles/17089/masked_keypoints.png}
\includegraphics[width=\textwidth]{appendix_figures/random_FDH/styleganL/singles/17098/masked_keypoints.png}
\includegraphics[width=\textwidth]{appendix_figures/random_FDH/styleganL/singles/17455/masked_keypoints.png}
\includegraphics[width=\textwidth]{appendix_figures/random_FDH/styleganL/singles/17591/masked_keypoints.png}
\caption{Condition}
\end{subfigure}%%
\begin{subfigure}[t]{0.125\textwidth}
\includegraphics[width=\textwidth]{appendix_figures/random_FDH/styleganL/singles/17043/fakes/0.png}
\includegraphics[width=\textwidth]{appendix_figures/random_FDH/styleganL/singles/17089/fakes/0.png}
\includegraphics[width=\textwidth]{appendix_figures/random_FDH/styleganL/singles/17098/fakes/0.png}
\includegraphics[width=\textwidth]{appendix_figures/random_FDH/styleganL/singles/17455/fakes/0.png}
\includegraphics[width=\textwidth]{appendix_figures/random_FDH/styleganL/singles/17591/fakes/0.png}
\caption{SG-GAN}
\end{subfigure}%%
\begin{subfigure}[t]{0.125\textwidth}
\includegraphics[width=\textwidth]{appendix_figures/random_FDH/styleganL/singles/17043/fakes/1.png}
\includegraphics[width=\textwidth]{appendix_figures/random_FDH/styleganL/singles/17089/fakes/1.png}
\includegraphics[width=\textwidth]{appendix_figures/random_FDH/styleganL/singles/17098/fakes/1.png}
\includegraphics[width=\textwidth]{appendix_figures/random_FDH/styleganL/singles/17455/fakes/1.png}
\includegraphics[width=\textwidth]{appendix_figures/random_FDH/styleganL/singles/17591/fakes/1.png}
\caption{SG-GAN}
\end{subfigure}%%
\begin{subfigure}[t]{0.125\textwidth}
\includegraphics[width=\textwidth]{appendix_figures/random_FDH/styleganL/singles/17043/fakes/2.png}
\includegraphics[width=\textwidth]{appendix_figures/random_FDH/styleganL/singles/17089/fakes/2.png}
\includegraphics[width=\textwidth]{appendix_figures/random_FDH/styleganL/singles/17098/fakes/2.png}
\includegraphics[width=\textwidth]{appendix_figures/random_FDH/styleganL/singles/17455/fakes/2.png}
\includegraphics[width=\textwidth]{appendix_figures/random_FDH/styleganL/singles/17591/fakes/2.png}
\caption{SG-GAN}
\end{subfigure}%%
\begin{subfigure}[t]{0.125\textwidth}
\includegraphics[width=\textwidth]{appendix_figures/random_FDH/im288/singles/17043/fakes/0.png}
\includegraphics[width=\textwidth]{appendix_figures/random_FDH/im288/singles/17089/fakes/0.png}
\includegraphics[width=\textwidth]{appendix_figures/random_FDH/im288/singles/17098/fakes/0.png}
\includegraphics[width=\textwidth]{appendix_figures/random_FDH/im288/singles/17455/fakes/0.png}
\includegraphics[width=\textwidth]{appendix_figures/random_FDH/im288/singles/17591/fakes/0.png}
\caption{\methodName}
\end{subfigure}%%
\begin{subfigure}[t]{0.125\textwidth}
\includegraphics[width=\textwidth]{appendix_figures/random_FDH/im288/singles/17043/fakes/1.png}
\includegraphics[width=\textwidth]{appendix_figures/random_FDH/im288/singles/17089/fakes/1.png}
\includegraphics[width=\textwidth]{appendix_figures/random_FDH/im288/singles/17098/fakes/1.png}
\includegraphics[width=\textwidth]{appendix_figures/random_FDH/im288/singles/17455/fakes/1.png}
\includegraphics[width=\textwidth]{appendix_figures/random_FDH/im288/singles/17591/fakes/1.png}
\caption{\methodName}
\end{subfigure}%%
\begin{subfigure}[t]{0.125\textwidth}
\includegraphics[width=\textwidth]{appendix_figures/random_FDH/im288/singles/17043/fakes/2.png}
\includegraphics[width=\textwidth]{appendix_figures/random_FDH/im288/singles/17089/fakes/2.png}
\includegraphics[width=\textwidth]{appendix_figures/random_FDH/im288/singles/17098/fakes/2.png}
\includegraphics[width=\textwidth]{appendix_figures/random_FDH/im288/singles/17455/fakes/2.png}
\includegraphics[width=\textwidth]{appendix_figures/random_FDH/im288/singles/17591/fakes/2.png}
\caption{\methodName}
\end{subfigure}%%
\caption{Random generated examples from FDH \cite{Hukkelas2022a} comparing \methodName to SG-GAN \cite{Hukkelas2022a}.
Note that all examples are generated with multi-modal truncation.
Surface map is not used by \methodName.}
\label{fig:fdh_random5}
\end{figure*}
\begin{figure*}[t]
\centering
\begin{subfigure}[t]{0.125\textwidth}
\includegraphics[width=\textwidth]{appendix_figures/random_FDH/styleganL/singles/18025/original.png}
\includegraphics[width=\textwidth]{appendix_figures/random_FDH/styleganL/singles/18430/original.png}
\includegraphics[width=\textwidth]{appendix_figures/random_FDH/styleganL/singles/18606/original.png}
\includegraphics[width=\textwidth]{appendix_figures/random_FDH/styleganL/singles/18635/original.png}
\includegraphics[width=\textwidth]{appendix_figures/random_FDH/styleganL/singles/18676/original.png}
\caption{Original}
\end{subfigure}%%
\begin{subfigure}[t]{0.125\textwidth}
\includegraphics[width=\textwidth]{appendix_figures/random_FDH/styleganL/singles/18025/masked_keypoints.png}
\includegraphics[width=\textwidth]{appendix_figures/random_FDH/styleganL/singles/18430/masked_keypoints.png}
\includegraphics[width=\textwidth]{appendix_figures/random_FDH/styleganL/singles/18606/masked_keypoints.png}
\includegraphics[width=\textwidth]{appendix_figures/random_FDH/styleganL/singles/18635/masked_keypoints.png}
\includegraphics[width=\textwidth]{appendix_figures/random_FDH/styleganL/singles/18676/masked_keypoints.png}
\caption{Condition}
\end{subfigure}%%
\begin{subfigure}[t]{0.125\textwidth}
\includegraphics[width=\textwidth]{appendix_figures/random_FDH/styleganL/singles/18025/fakes/0.png}
\includegraphics[width=\textwidth]{appendix_figures/random_FDH/styleganL/singles/18430/fakes/0.png}
\includegraphics[width=\textwidth]{appendix_figures/random_FDH/styleganL/singles/18606/fakes/0.png}
\includegraphics[width=\textwidth]{appendix_figures/random_FDH/styleganL/singles/18635/fakes/0.png}
\includegraphics[width=\textwidth]{appendix_figures/random_FDH/styleganL/singles/18676/fakes/0.png}
\caption{SG-GAN}
\end{subfigure}%%
\begin{subfigure}[t]{0.125\textwidth}
\includegraphics[width=\textwidth]{appendix_figures/random_FDH/styleganL/singles/18025/fakes/1.png}
\includegraphics[width=\textwidth]{appendix_figures/random_FDH/styleganL/singles/18430/fakes/1.png}
\includegraphics[width=\textwidth]{appendix_figures/random_FDH/styleganL/singles/18606/fakes/1.png}
\includegraphics[width=\textwidth]{appendix_figures/random_FDH/styleganL/singles/18635/fakes/1.png}
\includegraphics[width=\textwidth]{appendix_figures/random_FDH/styleganL/singles/18676/fakes/1.png}
\caption{SG-GAN}
\end{subfigure}%%
\begin{subfigure}[t]{0.125\textwidth}
\includegraphics[width=\textwidth]{appendix_figures/random_FDH/styleganL/singles/18025/fakes/2.png}
\includegraphics[width=\textwidth]{appendix_figures/random_FDH/styleganL/singles/18430/fakes/2.png}
\includegraphics[width=\textwidth]{appendix_figures/random_FDH/styleganL/singles/18606/fakes/2.png}
\includegraphics[width=\textwidth]{appendix_figures/random_FDH/styleganL/singles/18635/fakes/2.png}
\includegraphics[width=\textwidth]{appendix_figures/random_FDH/styleganL/singles/18676/fakes/2.png}
\caption{SG-GAN}
\end{subfigure}%%
\begin{subfigure}[t]{0.125\textwidth}
\includegraphics[width=\textwidth]{appendix_figures/random_FDH/im288/singles/18025/fakes/0.png}
\includegraphics[width=\textwidth]{appendix_figures/random_FDH/im288/singles/18430/fakes/0.png}
\includegraphics[width=\textwidth]{appendix_figures/random_FDH/im288/singles/18606/fakes/0.png}
\includegraphics[width=\textwidth]{appendix_figures/random_FDH/im288/singles/18635/fakes/0.png}
\includegraphics[width=\textwidth]{appendix_figures/random_FDH/im288/singles/18676/fakes/0.png}
\caption{\methodName}
\end{subfigure}%%
\begin{subfigure}[t]{0.125\textwidth}
\includegraphics[width=\textwidth]{appendix_figures/random_FDH/im288/singles/18025/fakes/1.png}
\includegraphics[width=\textwidth]{appendix_figures/random_FDH/im288/singles/18430/fakes/1.png}
\includegraphics[width=\textwidth]{appendix_figures/random_FDH/im288/singles/18606/fakes/1.png}
\includegraphics[width=\textwidth]{appendix_figures/random_FDH/im288/singles/18635/fakes/1.png}
\includegraphics[width=\textwidth]{appendix_figures/random_FDH/im288/singles/18676/fakes/1.png}
\caption{\methodName}
\end{subfigure}%%
\begin{subfigure}[t]{0.125\textwidth}
\includegraphics[width=\textwidth]{appendix_figures/random_FDH/im288/singles/18025/fakes/2.png}
\includegraphics[width=\textwidth]{appendix_figures/random_FDH/im288/singles/18430/fakes/2.png}
\includegraphics[width=\textwidth]{appendix_figures/random_FDH/im288/singles/18606/fakes/2.png}
\includegraphics[width=\textwidth]{appendix_figures/random_FDH/im288/singles/18635/fakes/2.png}
\includegraphics[width=\textwidth]{appendix_figures/random_FDH/im288/singles/18676/fakes/2.png}
\caption{\methodName}
\end{subfigure}%%
\caption{Random generated examples from FDH \cite{Hukkelas2022a} comparing \methodName to SG-GAN \cite{Hukkelas2022a}.
Note that all examples are generated with multi-modal truncation.
Surface map is not used by \methodName.}
\label{fig:fdh_random6}
\end{figure*}
\begin{figure*}[t]
\centering
\begin{subfigure}[t]{0.125\textwidth}
\includegraphics[width=\textwidth]{appendix_figures/random_FDH/styleganL/singles/19648/original.png}
\includegraphics[width=\textwidth]{appendix_figures/random_FDH/styleganL/singles/19721/original.png}
\includegraphics[width=\textwidth]{appendix_figures/random_FDH/styleganL/singles/19852/original.png}
\includegraphics[width=\textwidth]{appendix_figures/random_FDH/styleganL/singles/20006/original.png}
\includegraphics[width=\textwidth]{appendix_figures/random_FDH/styleganL/singles/20571/original.png}
\caption{Original}
\end{subfigure}%%
\begin{subfigure}[t]{0.125\textwidth}
\includegraphics[width=\textwidth]{appendix_figures/random_FDH/styleganL/singles/19648/masked_keypoints.png}
\includegraphics[width=\textwidth]{appendix_figures/random_FDH/styleganL/singles/19721/masked_keypoints.png}
\includegraphics[width=\textwidth]{appendix_figures/random_FDH/styleganL/singles/19852/masked_keypoints.png}
\includegraphics[width=\textwidth]{appendix_figures/random_FDH/styleganL/singles/20006/masked_keypoints.png}
\includegraphics[width=\textwidth]{appendix_figures/random_FDH/styleganL/singles/20571/masked_keypoints.png}
\caption{Condition}
\end{subfigure}%%
\begin{subfigure}[t]{0.125\textwidth}
\includegraphics[width=\textwidth]{appendix_figures/random_FDH/styleganL/singles/19648/fakes/0.png}
\includegraphics[width=\textwidth]{appendix_figures/random_FDH/styleganL/singles/19721/fakes/0.png}
\includegraphics[width=\textwidth]{appendix_figures/random_FDH/styleganL/singles/19852/fakes/0.png}
\includegraphics[width=\textwidth]{appendix_figures/random_FDH/styleganL/singles/20006/fakes/0.png}
\includegraphics[width=\textwidth]{appendix_figures/random_FDH/styleganL/singles/20571/fakes/0.png}
\caption{SG-GAN}
\end{subfigure}%%
\begin{subfigure}[t]{0.125\textwidth}
\includegraphics[width=\textwidth]{appendix_figures/random_FDH/styleganL/singles/19648/fakes/1.png}
\includegraphics[width=\textwidth]{appendix_figures/random_FDH/styleganL/singles/19721/fakes/1.png}
\includegraphics[width=\textwidth]{appendix_figures/random_FDH/styleganL/singles/19852/fakes/1.png}
\includegraphics[width=\textwidth]{appendix_figures/random_FDH/styleganL/singles/20006/fakes/1.png}
\includegraphics[width=\textwidth]{appendix_figures/random_FDH/styleganL/singles/20571/fakes/1.png}
\caption{SG-GAN}
\end{subfigure}%%
\begin{subfigure}[t]{0.125\textwidth}
\includegraphics[width=\textwidth]{appendix_figures/random_FDH/styleganL/singles/19648/fakes/2.png}
\includegraphics[width=\textwidth]{appendix_figures/random_FDH/styleganL/singles/19721/fakes/2.png}
\includegraphics[width=\textwidth]{appendix_figures/random_FDH/styleganL/singles/19852/fakes/2.png}
\includegraphics[width=\textwidth]{appendix_figures/random_FDH/styleganL/singles/20006/fakes/2.png}
\includegraphics[width=\textwidth]{appendix_figures/random_FDH/styleganL/singles/20571/fakes/2.png}
\caption{SG-GAN}
\end{subfigure}%%
\begin{subfigure}[t]{0.125\textwidth}
\includegraphics[width=\textwidth]{appendix_figures/random_FDH/im288/singles/19648/fakes/0.png}
\includegraphics[width=\textwidth]{appendix_figures/random_FDH/im288/singles/19721/fakes/0.png}
\includegraphics[width=\textwidth]{appendix_figures/random_FDH/im288/singles/19852/fakes/0.png}
\includegraphics[width=\textwidth]{appendix_figures/random_FDH/im288/singles/20006/fakes/0.png}
\includegraphics[width=\textwidth]{appendix_figures/random_FDH/im288/singles/20571/fakes/0.png}
\caption{\methodName}
\end{subfigure}%%
\begin{subfigure}[t]{0.125\textwidth}
\includegraphics[width=\textwidth]{appendix_figures/random_FDH/im288/singles/19648/fakes/1.png}
\includegraphics[width=\textwidth]{appendix_figures/random_FDH/im288/singles/19721/fakes/1.png}
\includegraphics[width=\textwidth]{appendix_figures/random_FDH/im288/singles/19852/fakes/1.png}
\includegraphics[width=\textwidth]{appendix_figures/random_FDH/im288/singles/20006/fakes/1.png}
\includegraphics[width=\textwidth]{appendix_figures/random_FDH/im288/singles/20571/fakes/1.png}
\caption{\methodName}
\end{subfigure}%%
\begin{subfigure}[t]{0.125\textwidth}
\includegraphics[width=\textwidth]{appendix_figures/random_FDH/im288/singles/19648/fakes/2.png}
\includegraphics[width=\textwidth]{appendix_figures/random_FDH/im288/singles/19721/fakes/2.png}
\includegraphics[width=\textwidth]{appendix_figures/random_FDH/im288/singles/19852/fakes/2.png}
\includegraphics[width=\textwidth]{appendix_figures/random_FDH/im288/singles/20006/fakes/2.png}
\includegraphics[width=\textwidth]{appendix_figures/random_FDH/im288/singles/20571/fakes/2.png}
\caption{\methodName}
\end{subfigure}%%
\caption{Random generated examples from FDH \cite{Hukkelas2022a} comparing \methodName to SG-GAN \cite{Hukkelas2022a}.
Note that all examples are generated with multi-modal truncation.
Surface map is not used by \methodName.}
\label{fig:fdh_random8}
\end{figure*}
\begin{figure*}[t]
\centering
\begin{subfigure}[t]{0.125\textwidth}
\includegraphics[width=\textwidth]{appendix_figures/random_FDH/styleganL/singles/20737/original.png}
\includegraphics[width=\textwidth]{appendix_figures/random_FDH/styleganL/singles/20757/original.png}
\includegraphics[width=\textwidth]{appendix_figures/random_FDH/styleganL/singles/21119/original.png}
\includegraphics[width=\textwidth]{appendix_figures/random_FDH/styleganL/singles/21243/original.png}
\includegraphics[width=\textwidth]{appendix_figures/random_FDH/styleganL/singles/21368/original.png}
\caption{Original}
\end{subfigure}%%
\begin{subfigure}[t]{0.125\textwidth}
\includegraphics[width=\textwidth]{appendix_figures/random_FDH/styleganL/singles/20737/masked_keypoints.png}
\includegraphics[width=\textwidth]{appendix_figures/random_FDH/styleganL/singles/20757/masked_keypoints.png}
\includegraphics[width=\textwidth]{appendix_figures/random_FDH/styleganL/singles/21119/masked_keypoints.png}
\includegraphics[width=\textwidth]{appendix_figures/random_FDH/styleganL/singles/21243/masked_keypoints.png}
\includegraphics[width=\textwidth]{appendix_figures/random_FDH/styleganL/singles/21368/masked_keypoints.png}
\caption{Condition}
\end{subfigure}%%
\begin{subfigure}[t]{0.125\textwidth}
\includegraphics[width=\textwidth]{appendix_figures/random_FDH/styleganL/singles/20737/fakes/0.png}
\includegraphics[width=\textwidth]{appendix_figures/random_FDH/styleganL/singles/20757/fakes/0.png}
\includegraphics[width=\textwidth]{appendix_figures/random_FDH/styleganL/singles/21119/fakes/0.png}
\includegraphics[width=\textwidth]{appendix_figures/random_FDH/styleganL/singles/21243/fakes/0.png}
\includegraphics[width=\textwidth]{appendix_figures/random_FDH/styleganL/singles/21368/fakes/0.png}
\caption{SG-GAN}
\end{subfigure}%%
\begin{subfigure}[t]{0.125\textwidth}
\includegraphics[width=\textwidth]{appendix_figures/random_FDH/styleganL/singles/20737/fakes/1.png}
\includegraphics[width=\textwidth]{appendix_figures/random_FDH/styleganL/singles/20757/fakes/1.png}
\includegraphics[width=\textwidth]{appendix_figures/random_FDH/styleganL/singles/21119/fakes/1.png}
\includegraphics[width=\textwidth]{appendix_figures/random_FDH/styleganL/singles/21243/fakes/1.png}
\includegraphics[width=\textwidth]{appendix_figures/random_FDH/styleganL/singles/21368/fakes/1.png}
\caption{SG-GAN}
\end{subfigure}%%
\begin{subfigure}[t]{0.125\textwidth}
\includegraphics[width=\textwidth]{appendix_figures/random_FDH/styleganL/singles/20737/fakes/2.png}
\includegraphics[width=\textwidth]{appendix_figures/random_FDH/styleganL/singles/20757/fakes/2.png}
\includegraphics[width=\textwidth]{appendix_figures/random_FDH/styleganL/singles/21119/fakes/2.png}
\includegraphics[width=\textwidth]{appendix_figures/random_FDH/styleganL/singles/21243/fakes/2.png}
\includegraphics[width=\textwidth]{appendix_figures/random_FDH/styleganL/singles/21368/fakes/2.png}
\caption{SG-GAN}
\end{subfigure}%%
\begin{subfigure}[t]{0.125\textwidth}
\includegraphics[width=\textwidth]{appendix_figures/random_FDH/im288/singles/20737/fakes/0.png}
\includegraphics[width=\textwidth]{appendix_figures/random_FDH/im288/singles/20757/fakes/0.png}
\includegraphics[width=\textwidth]{appendix_figures/random_FDH/im288/singles/21119/fakes/0.png}
\includegraphics[width=\textwidth]{appendix_figures/random_FDH/im288/singles/21243/fakes/0.png}
\includegraphics[width=\textwidth]{appendix_figures/random_FDH/im288/singles/21368/fakes/0.png}
\caption{\methodName}
\end{subfigure}%%
\begin{subfigure}[t]{0.125\textwidth}
\includegraphics[width=\textwidth]{appendix_figures/random_FDH/im288/singles/20737/fakes/1.png}
\includegraphics[width=\textwidth]{appendix_figures/random_FDH/im288/singles/20757/fakes/1.png}
\includegraphics[width=\textwidth]{appendix_figures/random_FDH/im288/singles/21119/fakes/1.png}
\includegraphics[width=\textwidth]{appendix_figures/random_FDH/im288/singles/21243/fakes/1.png}
\includegraphics[width=\textwidth]{appendix_figures/random_FDH/im288/singles/21368/fakes/1.png}
\caption{\methodName}
\end{subfigure}%%
\begin{subfigure}[t]{0.125\textwidth}
\includegraphics[width=\textwidth]{appendix_figures/random_FDH/im288/singles/20737/fakes/2.png}
\includegraphics[width=\textwidth]{appendix_figures/random_FDH/im288/singles/20757/fakes/2.png}
\includegraphics[width=\textwidth]{appendix_figures/random_FDH/im288/singles/21119/fakes/2.png}
\includegraphics[width=\textwidth]{appendix_figures/random_FDH/im288/singles/21243/fakes/2.png}
\includegraphics[width=\textwidth]{appendix_figures/random_FDH/im288/singles/21368/fakes/2.png}
\caption{\methodName}
\end{subfigure}%%
\caption{Random generated examples from FDH \cite{Hukkelas2022a} comparing \methodName to SG-GAN \cite{Hukkelas2022a}.
Note that all examples are generated with multi-modal truncation.
Surface map is not used by \methodName.}
\label{fig:fdh_random9}
\end{figure*}
\begin{figure*}[t]
\centering
\begin{subfigure}[t]{0.125\textwidth}
\includegraphics[width=\textwidth]{appendix_figures/random_FDH/styleganL/singles/2163/original.png}
\includegraphics[width=\textwidth]{appendix_figures/random_FDH/styleganL/singles/22258/original.png}
\includegraphics[width=\textwidth]{appendix_figures/random_FDH/styleganL/singles/22556/original.png}
\includegraphics[width=\textwidth]{appendix_figures/random_FDH/styleganL/singles/23071/original.png}
\includegraphics[width=\textwidth]{appendix_figures/random_FDH/styleganL/singles/23605/original.png}
\caption{Original}
\end{subfigure}%%
\begin{subfigure}[t]{0.125\textwidth}
\includegraphics[width=\textwidth]{appendix_figures/random_FDH/styleganL/singles/2163/masked_keypoints.png}
\includegraphics[width=\textwidth]{appendix_figures/random_FDH/styleganL/singles/22258/masked_keypoints.png}
\includegraphics[width=\textwidth]{appendix_figures/random_FDH/styleganL/singles/22556/masked_keypoints.png}
\includegraphics[width=\textwidth]{appendix_figures/random_FDH/styleganL/singles/23071/masked_keypoints.png}
\includegraphics[width=\textwidth]{appendix_figures/random_FDH/styleganL/singles/23605/masked_keypoints.png}
\caption{Condition}
\end{subfigure}%%
\begin{subfigure}[t]{0.125\textwidth}
\includegraphics[width=\textwidth]{appendix_figures/random_FDH/styleganL/singles/2163/fakes/0.png}
\includegraphics[width=\textwidth]{appendix_figures/random_FDH/styleganL/singles/22258/fakes/0.png}
\includegraphics[width=\textwidth]{appendix_figures/random_FDH/styleganL/singles/22556/fakes/0.png}
\includegraphics[width=\textwidth]{appendix_figures/random_FDH/styleganL/singles/23071/fakes/0.png}
\includegraphics[width=\textwidth]{appendix_figures/random_FDH/styleganL/singles/23605/fakes/0.png}
\caption{SG-GAN}
\end{subfigure}%%
\begin{subfigure}[t]{0.125\textwidth}
\includegraphics[width=\textwidth]{appendix_figures/random_FDH/styleganL/singles/2163/fakes/1.png}
\includegraphics[width=\textwidth]{appendix_figures/random_FDH/styleganL/singles/22258/fakes/1.png}
\includegraphics[width=\textwidth]{appendix_figures/random_FDH/styleganL/singles/22556/fakes/1.png}
\includegraphics[width=\textwidth]{appendix_figures/random_FDH/styleganL/singles/23071/fakes/1.png}
\includegraphics[width=\textwidth]{appendix_figures/random_FDH/styleganL/singles/23605/fakes/1.png}
\caption{SG-GAN}
\end{subfigure}%%
\begin{subfigure}[t]{0.125\textwidth}
\includegraphics[width=\textwidth]{appendix_figures/random_FDH/styleganL/singles/2163/fakes/2.png}
\includegraphics[width=\textwidth]{appendix_figures/random_FDH/styleganL/singles/22258/fakes/2.png}
\includegraphics[width=\textwidth]{appendix_figures/random_FDH/styleganL/singles/22556/fakes/2.png}
\includegraphics[width=\textwidth]{appendix_figures/random_FDH/styleganL/singles/23071/fakes/2.png}
\includegraphics[width=\textwidth]{appendix_figures/random_FDH/styleganL/singles/23605/fakes/2.png}
\caption{SG-GAN}
\end{subfigure}%%
\begin{subfigure}[t]{0.125\textwidth}
\includegraphics[width=\textwidth]{appendix_figures/random_FDH/im288/singles/2163/fakes/0.png}
\includegraphics[width=\textwidth]{appendix_figures/random_FDH/im288/singles/22258/fakes/0.png}
\includegraphics[width=\textwidth]{appendix_figures/random_FDH/im288/singles/22556/fakes/0.png}
\includegraphics[width=\textwidth]{appendix_figures/random_FDH/im288/singles/23071/fakes/0.png}
\includegraphics[width=\textwidth]{appendix_figures/random_FDH/im288/singles/23605/fakes/0.png}
\caption{\methodName}
\end{subfigure}%%
\begin{subfigure}[t]{0.125\textwidth}
\includegraphics[width=\textwidth]{appendix_figures/random_FDH/im288/singles/2163/fakes/1.png}
\includegraphics[width=\textwidth]{appendix_figures/random_FDH/im288/singles/22258/fakes/1.png}
\includegraphics[width=\textwidth]{appendix_figures/random_FDH/im288/singles/22556/fakes/1.png}
\includegraphics[width=\textwidth]{appendix_figures/random_FDH/im288/singles/23071/fakes/1.png}
\includegraphics[width=\textwidth]{appendix_figures/random_FDH/im288/singles/23605/fakes/1.png}
\caption{\methodName}
\end{subfigure}%%
\begin{subfigure}[t]{0.125\textwidth}
\includegraphics[width=\textwidth]{appendix_figures/random_FDH/im288/singles/2163/fakes/2.png}
\includegraphics[width=\textwidth]{appendix_figures/random_FDH/im288/singles/22258/fakes/2.png}
\includegraphics[width=\textwidth]{appendix_figures/random_FDH/im288/singles/22556/fakes/2.png}
\includegraphics[width=\textwidth]{appendix_figures/random_FDH/im288/singles/23071/fakes/2.png}
\includegraphics[width=\textwidth]{appendix_figures/random_FDH/im288/singles/23605/fakes/2.png}
\caption{\methodName}
\end{subfigure}%%
\caption{Random generated examples from FDH \cite{Hukkelas2022a} comparing \methodName to SG-GAN \cite{Hukkelas2022a}.
Note that all examples are generated with multi-modal truncation.
Surface map is not used by \methodName.}
\label{fig:fdh_random10}
\end{figure*}
\begin{figure*}[t]
\centering
\begin{subfigure}[t]{0.125\textwidth}
\includegraphics[width=\textwidth]{appendix_figures/random_FDH/styleganL/singles/23634/original.png}
\includegraphics[width=\textwidth]{appendix_figures/random_FDH/styleganL/singles/23840/original.png}
\includegraphics[width=\textwidth]{appendix_figures/random_FDH/styleganL/singles/24152/original.png}
\includegraphics[width=\textwidth]{appendix_figures/random_FDH/styleganL/singles/24275/original.png}
\includegraphics[width=\textwidth]{appendix_figures/random_FDH/styleganL/singles/24675/original.png}
\caption{Original}
\end{subfigure}%%
\begin{subfigure}[t]{0.125\textwidth}
\includegraphics[width=\textwidth]{appendix_figures/random_FDH/styleganL/singles/23634/masked_keypoints.png}
\includegraphics[width=\textwidth]{appendix_figures/random_FDH/styleganL/singles/23840/masked_keypoints.png}
\includegraphics[width=\textwidth]{appendix_figures/random_FDH/styleganL/singles/24152/masked_keypoints.png}
\includegraphics[width=\textwidth]{appendix_figures/random_FDH/styleganL/singles/24275/masked_keypoints.png}
\includegraphics[width=\textwidth]{appendix_figures/random_FDH/styleganL/singles/24675/masked_keypoints.png}
\caption{Condition}
\end{subfigure}%%
\begin{subfigure}[t]{0.125\textwidth}
\includegraphics[width=\textwidth]{appendix_figures/random_FDH/styleganL/singles/23634/fakes/0.png}
\includegraphics[width=\textwidth]{appendix_figures/random_FDH/styleganL/singles/23840/fakes/0.png}
\includegraphics[width=\textwidth]{appendix_figures/random_FDH/styleganL/singles/24152/fakes/0.png}
\includegraphics[width=\textwidth]{appendix_figures/random_FDH/styleganL/singles/24275/fakes/0.png}
\includegraphics[width=\textwidth]{appendix_figures/random_FDH/styleganL/singles/24675/fakes/0.png}
\caption{SG-GAN}
\end{subfigure}%%
\begin{subfigure}[t]{0.125\textwidth}
\includegraphics[width=\textwidth]{appendix_figures/random_FDH/styleganL/singles/23634/fakes/1.png}
\includegraphics[width=\textwidth]{appendix_figures/random_FDH/styleganL/singles/23840/fakes/1.png}
\includegraphics[width=\textwidth]{appendix_figures/random_FDH/styleganL/singles/24152/fakes/1.png}
\includegraphics[width=\textwidth]{appendix_figures/random_FDH/styleganL/singles/24275/fakes/1.png}
\includegraphics[width=\textwidth]{appendix_figures/random_FDH/styleganL/singles/24675/fakes/1.png}
\caption{SG-GAN}
\end{subfigure}%%
\begin{subfigure}[t]{0.125\textwidth}
\includegraphics[width=\textwidth]{appendix_figures/random_FDH/styleganL/singles/23634/fakes/2.png}
\includegraphics[width=\textwidth]{appendix_figures/random_FDH/styleganL/singles/23840/fakes/2.png}
\includegraphics[width=\textwidth]{appendix_figures/random_FDH/styleganL/singles/24152/fakes/2.png}
\includegraphics[width=\textwidth]{appendix_figures/random_FDH/styleganL/singles/24275/fakes/2.png}
\includegraphics[width=\textwidth]{appendix_figures/random_FDH/styleganL/singles/24675/fakes/2.png}
\caption{SG-GAN}
\end{subfigure}%%
\begin{subfigure}[t]{0.125\textwidth}
\includegraphics[width=\textwidth]{appendix_figures/random_FDH/im288/singles/23634/fakes/0.png}
\includegraphics[width=\textwidth]{appendix_figures/random_FDH/im288/singles/23840/fakes/0.png}
\includegraphics[width=\textwidth]{appendix_figures/random_FDH/im288/singles/24152/fakes/0.png}
\includegraphics[width=\textwidth]{appendix_figures/random_FDH/im288/singles/24275/fakes/0.png}
\includegraphics[width=\textwidth]{appendix_figures/random_FDH/im288/singles/24675/fakes/0.png}
\caption{\methodName}
\end{subfigure}%%
\begin{subfigure}[t]{0.125\textwidth}
\includegraphics[width=\textwidth]{appendix_figures/random_FDH/im288/singles/23634/fakes/1.png}
\includegraphics[width=\textwidth]{appendix_figures/random_FDH/im288/singles/23840/fakes/1.png}
\includegraphics[width=\textwidth]{appendix_figures/random_FDH/im288/singles/24152/fakes/1.png}
\includegraphics[width=\textwidth]{appendix_figures/random_FDH/im288/singles/24275/fakes/1.png}
\includegraphics[width=\textwidth]{appendix_figures/random_FDH/im288/singles/24675/fakes/1.png}
\caption{\methodName}
\end{subfigure}%%
\begin{subfigure}[t]{0.125\textwidth}
\includegraphics[width=\textwidth]{appendix_figures/random_FDH/im288/singles/23634/fakes/2.png}
\includegraphics[width=\textwidth]{appendix_figures/random_FDH/im288/singles/23840/fakes/2.png}
\includegraphics[width=\textwidth]{appendix_figures/random_FDH/im288/singles/24152/fakes/2.png}
\includegraphics[width=\textwidth]{appendix_figures/random_FDH/im288/singles/24275/fakes/2.png}
\includegraphics[width=\textwidth]{appendix_figures/random_FDH/im288/singles/24675/fakes/2.png}
\caption{\methodName}
\end{subfigure}%%
\caption{Random generated examples from FDH \cite{Hukkelas2022a} comparing \methodName to SG-GAN \cite{Hukkelas2022a}.
Note that all examples are generated with multi-modal truncation.
Surface map is not used by \methodName.}
\label{fig:fdh_random11}
\end{figure*}
\begin{figure*}[t]
\centering
\begin{subfigure}[t]{0.125\textwidth}
\includegraphics[width=\textwidth]{appendix_figures/random_FDH/styleganL/singles/24727/original.png}
\includegraphics[width=\textwidth]{appendix_figures/random_FDH/styleganL/singles/2496/original.png}
\includegraphics[width=\textwidth]{appendix_figures/random_FDH/styleganL/singles/24999/original.png}
\includegraphics[width=\textwidth]{appendix_figures/random_FDH/styleganL/singles/25332/original.png}
\includegraphics[width=\textwidth]{appendix_figures/random_FDH/styleganL/singles/25378/original.png}
\caption{Original}
\end{subfigure}%%
\begin{subfigure}[t]{0.125\textwidth}
\includegraphics[width=\textwidth]{appendix_figures/random_FDH/styleganL/singles/24727/masked_keypoints.png}
\includegraphics[width=\textwidth]{appendix_figures/random_FDH/styleganL/singles/2496/masked_keypoints.png}
\includegraphics[width=\textwidth]{appendix_figures/random_FDH/styleganL/singles/24999/masked_keypoints.png}
\includegraphics[width=\textwidth]{appendix_figures/random_FDH/styleganL/singles/25332/masked_keypoints.png}
\includegraphics[width=\textwidth]{appendix_figures/random_FDH/styleganL/singles/25378/masked_keypoints.png}
\caption{Condition}
\end{subfigure}%%
\begin{subfigure}[t]{0.125\textwidth}
\includegraphics[width=\textwidth]{appendix_figures/random_FDH/styleganL/singles/24727/fakes/0.png}
\includegraphics[width=\textwidth]{appendix_figures/random_FDH/styleganL/singles/2496/fakes/0.png}
\includegraphics[width=\textwidth]{appendix_figures/random_FDH/styleganL/singles/24999/fakes/0.png}
\includegraphics[width=\textwidth]{appendix_figures/random_FDH/styleganL/singles/25332/fakes/0.png}
\includegraphics[width=\textwidth]{appendix_figures/random_FDH/styleganL/singles/25378/fakes/0.png}
\caption{SG-GAN}
\end{subfigure}%%
\begin{subfigure}[t]{0.125\textwidth}
\includegraphics[width=\textwidth]{appendix_figures/random_FDH/styleganL/singles/24727/fakes/1.png}
\includegraphics[width=\textwidth]{appendix_figures/random_FDH/styleganL/singles/2496/fakes/1.png}
\includegraphics[width=\textwidth]{appendix_figures/random_FDH/styleganL/singles/24999/fakes/1.png}
\includegraphics[width=\textwidth]{appendix_figures/random_FDH/styleganL/singles/25332/fakes/1.png}
\includegraphics[width=\textwidth]{appendix_figures/random_FDH/styleganL/singles/25378/fakes/1.png}
\caption{SG-GAN}
\end{subfigure}%%
\begin{subfigure}[t]{0.125\textwidth}
\includegraphics[width=\textwidth]{appendix_figures/random_FDH/styleganL/singles/24727/fakes/2.png}
\includegraphics[width=\textwidth]{appendix_figures/random_FDH/styleganL/singles/2496/fakes/2.png}
\includegraphics[width=\textwidth]{appendix_figures/random_FDH/styleganL/singles/24999/fakes/2.png}
\includegraphics[width=\textwidth]{appendix_figures/random_FDH/styleganL/singles/25332/fakes/2.png}
\includegraphics[width=\textwidth]{appendix_figures/random_FDH/styleganL/singles/25378/fakes/2.png}
\caption{SG-GAN}
\end{subfigure}%%
\begin{subfigure}[t]{0.125\textwidth}
\includegraphics[width=\textwidth]{appendix_figures/random_FDH/im288/singles/24727/fakes/0.png}
\includegraphics[width=\textwidth]{appendix_figures/random_FDH/im288/singles/2496/fakes/0.png}
\includegraphics[width=\textwidth]{appendix_figures/random_FDH/im288/singles/24999/fakes/0.png}
\includegraphics[width=\textwidth]{appendix_figures/random_FDH/im288/singles/25332/fakes/0.png}
\includegraphics[width=\textwidth]{appendix_figures/random_FDH/im288/singles/25378/fakes/0.png}
\caption{\methodName}
\end{subfigure}%%
\begin{subfigure}[t]{0.125\textwidth}
\includegraphics[width=\textwidth]{appendix_figures/random_FDH/im288/singles/24727/fakes/1.png}
\includegraphics[width=\textwidth]{appendix_figures/random_FDH/im288/singles/2496/fakes/1.png}
\includegraphics[width=\textwidth]{appendix_figures/random_FDH/im288/singles/24999/fakes/1.png}
\includegraphics[width=\textwidth]{appendix_figures/random_FDH/im288/singles/25332/fakes/1.png}
\includegraphics[width=\textwidth]{appendix_figures/random_FDH/im288/singles/25378/fakes/1.png}
\caption{\methodName}
\end{subfigure}%%
\begin{subfigure}[t]{0.125\textwidth}
\includegraphics[width=\textwidth]{appendix_figures/random_FDH/im288/singles/24727/fakes/2.png}
\includegraphics[width=\textwidth]{appendix_figures/random_FDH/im288/singles/2496/fakes/2.png}
\includegraphics[width=\textwidth]{appendix_figures/random_FDH/im288/singles/24999/fakes/2.png}
\includegraphics[width=\textwidth]{appendix_figures/random_FDH/im288/singles/25332/fakes/2.png}
\includegraphics[width=\textwidth]{appendix_figures/random_FDH/im288/singles/25378/fakes/2.png}
\caption{\methodName}
\end{subfigure}%%
\caption{Random generated examples from FDH \cite{Hukkelas2022a} comparing \methodName to SG-GAN \cite{Hukkelas2022a}.
Note that all examples are generated with multi-modal truncation.
Surface map is not used by \methodName.}
\label{fig:fdh_random12}
\end{figure*}
\begin{figure*}[t]
\centering
\begin{subfigure}[t]{0.125\textwidth}
\includegraphics[width=\textwidth]{appendix_figures/random_FDH/styleganL/singles/26277/original.png}
\includegraphics[width=\textwidth]{appendix_figures/random_FDH/styleganL/singles/26532/original.png}
\includegraphics[width=\textwidth]{appendix_figures/random_FDH/styleganL/singles/26681/original.png}
\includegraphics[width=\textwidth]{appendix_figures/random_FDH/styleganL/singles/26752/original.png}
\includegraphics[width=\textwidth]{appendix_figures/random_FDH/styleganL/singles/27022/original.png}
\caption{Original}
\end{subfigure}%%
\begin{subfigure}[t]{0.125\textwidth}
\includegraphics[width=\textwidth]{appendix_figures/random_FDH/styleganL/singles/26277/masked_keypoints.png}
\includegraphics[width=\textwidth]{appendix_figures/random_FDH/styleganL/singles/26532/masked_keypoints.png}
\includegraphics[width=\textwidth]{appendix_figures/random_FDH/styleganL/singles/26681/masked_keypoints.png}
\includegraphics[width=\textwidth]{appendix_figures/random_FDH/styleganL/singles/26752/masked_keypoints.png}
\includegraphics[width=\textwidth]{appendix_figures/random_FDH/styleganL/singles/27022/masked_keypoints.png}
\caption{Condition}
\end{subfigure}%%
\begin{subfigure}[t]{0.125\textwidth}
\includegraphics[width=\textwidth]{appendix_figures/random_FDH/styleganL/singles/26277/fakes/0.png}
\includegraphics[width=\textwidth]{appendix_figures/random_FDH/styleganL/singles/26532/fakes/0.png}
\includegraphics[width=\textwidth]{appendix_figures/random_FDH/styleganL/singles/26681/fakes/0.png}
\includegraphics[width=\textwidth]{appendix_figures/random_FDH/styleganL/singles/26752/fakes/0.png}
\includegraphics[width=\textwidth]{appendix_figures/random_FDH/styleganL/singles/27022/fakes/0.png}
\caption{SG-GAN}
\end{subfigure}%%
\begin{subfigure}[t]{0.125\textwidth}
\includegraphics[width=\textwidth]{appendix_figures/random_FDH/styleganL/singles/26277/fakes/1.png}
\includegraphics[width=\textwidth]{appendix_figures/random_FDH/styleganL/singles/26532/fakes/1.png}
\includegraphics[width=\textwidth]{appendix_figures/random_FDH/styleganL/singles/26681/fakes/1.png}
\includegraphics[width=\textwidth]{appendix_figures/random_FDH/styleganL/singles/26752/fakes/1.png}
\includegraphics[width=\textwidth]{appendix_figures/random_FDH/styleganL/singles/27022/fakes/1.png}
\caption{SG-GAN}
\end{subfigure}%%
\begin{subfigure}[t]{0.125\textwidth}
\includegraphics[width=\textwidth]{appendix_figures/random_FDH/styleganL/singles/26277/fakes/2.png}
\includegraphics[width=\textwidth]{appendix_figures/random_FDH/styleganL/singles/26532/fakes/2.png}
\includegraphics[width=\textwidth]{appendix_figures/random_FDH/styleganL/singles/26681/fakes/2.png}
\includegraphics[width=\textwidth]{appendix_figures/random_FDH/styleganL/singles/26752/fakes/2.png}
\includegraphics[width=\textwidth]{appendix_figures/random_FDH/styleganL/singles/27022/fakes/2.png}
\caption{SG-GAN}
\end{subfigure}%%
\begin{subfigure}[t]{0.125\textwidth}
\includegraphics[width=\textwidth]{appendix_figures/random_FDH/im288/singles/26277/fakes/0.png}
\includegraphics[width=\textwidth]{appendix_figures/random_FDH/im288/singles/26532/fakes/0.png}
\includegraphics[width=\textwidth]{appendix_figures/random_FDH/im288/singles/26681/fakes/0.png}
\includegraphics[width=\textwidth]{appendix_figures/random_FDH/im288/singles/26752/fakes/0.png}
\includegraphics[width=\textwidth]{appendix_figures/random_FDH/im288/singles/27022/fakes/0.png}
\caption{\methodName}
\end{subfigure}%%
\begin{subfigure}[t]{0.125\textwidth}
\includegraphics[width=\textwidth]{appendix_figures/random_FDH/im288/singles/26277/fakes/1.png}
\includegraphics[width=\textwidth]{appendix_figures/random_FDH/im288/singles/26532/fakes/1.png}
\includegraphics[width=\textwidth]{appendix_figures/random_FDH/im288/singles/26681/fakes/1.png}
\includegraphics[width=\textwidth]{appendix_figures/random_FDH/im288/singles/26752/fakes/1.png}
\includegraphics[width=\textwidth]{appendix_figures/random_FDH/im288/singles/27022/fakes/1.png}
\caption{\methodName}
\end{subfigure}%%
\begin{subfigure}[t]{0.125\textwidth}
\includegraphics[width=\textwidth]{appendix_figures/random_FDH/im288/singles/26277/fakes/2.png}
\includegraphics[width=\textwidth]{appendix_figures/random_FDH/im288/singles/26532/fakes/2.png}
\includegraphics[width=\textwidth]{appendix_figures/random_FDH/im288/singles/26681/fakes/2.png}
\includegraphics[width=\textwidth]{appendix_figures/random_FDH/im288/singles/26752/fakes/2.png}
\includegraphics[width=\textwidth]{appendix_figures/random_FDH/im288/singles/27022/fakes/2.png}
\caption{\methodName}
\end{subfigure}%%
\caption{Random generated examples from FDH \cite{Hukkelas2022a} comparing \methodName to SG-GAN \cite{Hukkelas2022a}.
Note that all examples are generated with multi-modal truncation.
Surface map is not used by \methodName.}
\label{fig:fdh_random13}
\end{figure*}
\begin{figure*}[t]
\centering
\begin{subfigure}[t]{0.125\textwidth}
\includegraphics[width=\textwidth]{appendix_figures/random_FDH/styleganL/singles/27257/original.png}
\includegraphics[width=\textwidth]{appendix_figures/random_FDH/styleganL/singles/27299/original.png}
\includegraphics[width=\textwidth]{appendix_figures/random_FDH/styleganL/singles/2732/original.png}
\includegraphics[width=\textwidth]{appendix_figures/random_FDH/styleganL/singles/27469/original.png}
\includegraphics[width=\textwidth]{appendix_figures/random_FDH/styleganL/singles/27690/original.png}
\caption{Original}
\end{subfigure}%%
\begin{subfigure}[t]{0.125\textwidth}
\includegraphics[width=\textwidth]{appendix_figures/random_FDH/styleganL/singles/27257/masked_keypoints.png}
\includegraphics[width=\textwidth]{appendix_figures/random_FDH/styleganL/singles/27299/masked_keypoints.png}
\includegraphics[width=\textwidth]{appendix_figures/random_FDH/styleganL/singles/2732/masked_keypoints.png}
\includegraphics[width=\textwidth]{appendix_figures/random_FDH/styleganL/singles/27469/masked_keypoints.png}
\includegraphics[width=\textwidth]{appendix_figures/random_FDH/styleganL/singles/27690/masked_keypoints.png}
\caption{Condition}
\end{subfigure}%%
\begin{subfigure}[t]{0.125\textwidth}
\includegraphics[width=\textwidth]{appendix_figures/random_FDH/styleganL/singles/27257/fakes/0.png}
\includegraphics[width=\textwidth]{appendix_figures/random_FDH/styleganL/singles/27299/fakes/0.png}
\includegraphics[width=\textwidth]{appendix_figures/random_FDH/styleganL/singles/2732/fakes/0.png}
\includegraphics[width=\textwidth]{appendix_figures/random_FDH/styleganL/singles/27469/fakes/0.png}
\includegraphics[width=\textwidth]{appendix_figures/random_FDH/styleganL/singles/27690/fakes/0.png}
\caption{SG-GAN}
\end{subfigure}%%
\begin{subfigure}[t]{0.125\textwidth}
\includegraphics[width=\textwidth]{appendix_figures/random_FDH/styleganL/singles/27257/fakes/1.png}
\includegraphics[width=\textwidth]{appendix_figures/random_FDH/styleganL/singles/27299/fakes/1.png}
\includegraphics[width=\textwidth]{appendix_figures/random_FDH/styleganL/singles/2732/fakes/1.png}
\includegraphics[width=\textwidth]{appendix_figures/random_FDH/styleganL/singles/27469/fakes/1.png}
\includegraphics[width=\textwidth]{appendix_figures/random_FDH/styleganL/singles/27690/fakes/1.png}
\caption{SG-GAN}
\end{subfigure}%%
\begin{subfigure}[t]{0.125\textwidth}
\includegraphics[width=\textwidth]{appendix_figures/random_FDH/styleganL/singles/27257/fakes/2.png}
\includegraphics[width=\textwidth]{appendix_figures/random_FDH/styleganL/singles/27299/fakes/2.png}
\includegraphics[width=\textwidth]{appendix_figures/random_FDH/styleganL/singles/2732/fakes/2.png}
\includegraphics[width=\textwidth]{appendix_figures/random_FDH/styleganL/singles/27469/fakes/2.png}
\includegraphics[width=\textwidth]{appendix_figures/random_FDH/styleganL/singles/27690/fakes/2.png}
\caption{SG-GAN}
\end{subfigure}%%
\begin{subfigure}[t]{0.125\textwidth}
\includegraphics[width=\textwidth]{appendix_figures/random_FDH/im288/singles/27257/fakes/0.png}
\includegraphics[width=\textwidth]{appendix_figures/random_FDH/im288/singles/27299/fakes/0.png}
\includegraphics[width=\textwidth]{appendix_figures/random_FDH/im288/singles/2732/fakes/0.png}
\includegraphics[width=\textwidth]{appendix_figures/random_FDH/im288/singles/27469/fakes/0.png}
\includegraphics[width=\textwidth]{appendix_figures/random_FDH/im288/singles/27690/fakes/0.png}
\caption{\methodName}
\end{subfigure}%%
\begin{subfigure}[t]{0.125\textwidth}
\includegraphics[width=\textwidth]{appendix_figures/random_FDH/im288/singles/27257/fakes/1.png}
\includegraphics[width=\textwidth]{appendix_figures/random_FDH/im288/singles/27299/fakes/1.png}
\includegraphics[width=\textwidth]{appendix_figures/random_FDH/im288/singles/2732/fakes/1.png}
\includegraphics[width=\textwidth]{appendix_figures/random_FDH/im288/singles/27469/fakes/1.png}
\includegraphics[width=\textwidth]{appendix_figures/random_FDH/im288/singles/27690/fakes/1.png}
\caption{\methodName}
\end{subfigure}%%
\begin{subfigure}[t]{0.125\textwidth}
\includegraphics[width=\textwidth]{appendix_figures/random_FDH/im288/singles/27257/fakes/2.png}
\includegraphics[width=\textwidth]{appendix_figures/random_FDH/im288/singles/27299/fakes/2.png}
\includegraphics[width=\textwidth]{appendix_figures/random_FDH/im288/singles/2732/fakes/2.png}
\includegraphics[width=\textwidth]{appendix_figures/random_FDH/im288/singles/27469/fakes/2.png}
\includegraphics[width=\textwidth]{appendix_figures/random_FDH/im288/singles/27690/fakes/2.png}
\caption{\methodName}
\end{subfigure}%%
\caption{Random generated examples from FDH \cite{Hukkelas2022a} comparing \methodName to SG-GAN \cite{Hukkelas2022a}.
Note that all examples are generated with multi-modal truncation.
Surface map is not used by \methodName.}
\label{fig:fdh_random14}
\end{figure*}
\begin{figure*}[t]
\centering
\begin{subfigure}[t]{0.125\textwidth}
\includegraphics[width=\textwidth]{appendix_figures/random_FDH/styleganL/singles/27767/original.png}
\includegraphics[width=\textwidth]{appendix_figures/random_FDH/styleganL/singles/28585/original.png}
\includegraphics[width=\textwidth]{appendix_figures/random_FDH/styleganL/singles/28647/original.png}
\includegraphics[width=\textwidth]{appendix_figures/random_FDH/styleganL/singles/28945/original.png}
\includegraphics[width=\textwidth]{appendix_figures/random_FDH/styleganL/singles/2897/original.png}
\caption{Original}
\end{subfigure}%%
\begin{subfigure}[t]{0.125\textwidth}
\includegraphics[width=\textwidth]{appendix_figures/random_FDH/styleganL/singles/27767/masked_keypoints.png}
\includegraphics[width=\textwidth]{appendix_figures/random_FDH/styleganL/singles/28585/masked_keypoints.png}
\includegraphics[width=\textwidth]{appendix_figures/random_FDH/styleganL/singles/28647/masked_keypoints.png}
\includegraphics[width=\textwidth]{appendix_figures/random_FDH/styleganL/singles/28945/masked_keypoints.png}
\includegraphics[width=\textwidth]{appendix_figures/random_FDH/styleganL/singles/2897/masked_keypoints.png}
\caption{Condition}
\end{subfigure}%%
\begin{subfigure}[t]{0.125\textwidth}
\includegraphics[width=\textwidth]{appendix_figures/random_FDH/styleganL/singles/27767/fakes/0.png}
\includegraphics[width=\textwidth]{appendix_figures/random_FDH/styleganL/singles/28585/fakes/0.png}
\includegraphics[width=\textwidth]{appendix_figures/random_FDH/styleganL/singles/28647/fakes/0.png}
\includegraphics[width=\textwidth]{appendix_figures/random_FDH/styleganL/singles/28945/fakes/0.png}
\includegraphics[width=\textwidth]{appendix_figures/random_FDH/styleganL/singles/2897/fakes/0.png}
\caption{SG-GAN}
\end{subfigure}%%
\begin{subfigure}[t]{0.125\textwidth}
\includegraphics[width=\textwidth]{appendix_figures/random_FDH/styleganL/singles/27767/fakes/1.png}
\includegraphics[width=\textwidth]{appendix_figures/random_FDH/styleganL/singles/28585/fakes/1.png}
\includegraphics[width=\textwidth]{appendix_figures/random_FDH/styleganL/singles/28647/fakes/1.png}
\includegraphics[width=\textwidth]{appendix_figures/random_FDH/styleganL/singles/28945/fakes/1.png}
\includegraphics[width=\textwidth]{appendix_figures/random_FDH/styleganL/singles/2897/fakes/1.png}
\caption{SG-GAN}
\end{subfigure}%%
\begin{subfigure}[t]{0.125\textwidth}
\includegraphics[width=\textwidth]{appendix_figures/random_FDH/styleganL/singles/27767/fakes/2.png}
\includegraphics[width=\textwidth]{appendix_figures/random_FDH/styleganL/singles/28585/fakes/2.png}
\includegraphics[width=\textwidth]{appendix_figures/random_FDH/styleganL/singles/28647/fakes/2.png}
\includegraphics[width=\textwidth]{appendix_figures/random_FDH/styleganL/singles/28945/fakes/2.png}
\includegraphics[width=\textwidth]{appendix_figures/random_FDH/styleganL/singles/2897/fakes/2.png}
\caption{SG-GAN}
\end{subfigure}%%
\begin{subfigure}[t]{0.125\textwidth}
\includegraphics[width=\textwidth]{appendix_figures/random_FDH/im288/singles/27767/fakes/0.png}
\includegraphics[width=\textwidth]{appendix_figures/random_FDH/im288/singles/28585/fakes/0.png}
\includegraphics[width=\textwidth]{appendix_figures/random_FDH/im288/singles/28647/fakes/0.png}
\includegraphics[width=\textwidth]{appendix_figures/random_FDH/im288/singles/28945/fakes/0.png}
\includegraphics[width=\textwidth]{appendix_figures/random_FDH/im288/singles/2897/fakes/0.png}
\caption{\methodName}
\end{subfigure}%%
\begin{subfigure}[t]{0.125\textwidth}
\includegraphics[width=\textwidth]{appendix_figures/random_FDH/im288/singles/27767/fakes/1.png}
\includegraphics[width=\textwidth]{appendix_figures/random_FDH/im288/singles/28585/fakes/1.png}
\includegraphics[width=\textwidth]{appendix_figures/random_FDH/im288/singles/28647/fakes/1.png}
\includegraphics[width=\textwidth]{appendix_figures/random_FDH/im288/singles/28945/fakes/1.png}
\includegraphics[width=\textwidth]{appendix_figures/random_FDH/im288/singles/2897/fakes/1.png}
\caption{\methodName}
\end{subfigure}%%
\begin{subfigure}[t]{0.125\textwidth}
\includegraphics[width=\textwidth]{appendix_figures/random_FDH/im288/singles/27767/fakes/2.png}
\includegraphics[width=\textwidth]{appendix_figures/random_FDH/im288/singles/28585/fakes/2.png}
\includegraphics[width=\textwidth]{appendix_figures/random_FDH/im288/singles/28647/fakes/2.png}
\includegraphics[width=\textwidth]{appendix_figures/random_FDH/im288/singles/28945/fakes/2.png}
\includegraphics[width=\textwidth]{appendix_figures/random_FDH/im288/singles/2897/fakes/2.png}
\caption{\methodName}
\end{subfigure}%%
\caption{Random generated examples from FDH \cite{Hukkelas2022a} comparing \methodName to SG-GAN \cite{Hukkelas2022a}.
Note that all examples are generated with multi-modal truncation.
Surface map is not used by \methodName.}
\label{fig:fdh_random15}
\end{figure*}
\begin{figure*}[t]
\centering
\begin{subfigure}[t]{0.125\textwidth}
\includegraphics[width=\textwidth]{appendix_figures/random_FDH/styleganL/singles/3219/original.png}
\includegraphics[width=\textwidth]{appendix_figures/random_FDH/styleganL/singles/3560/original.png}
\includegraphics[width=\textwidth]{appendix_figures/random_FDH/styleganL/singles/4420/original.png}
\includegraphics[width=\textwidth]{appendix_figures/random_FDH/styleganL/singles/4851/original.png}
\includegraphics[width=\textwidth]{appendix_figures/random_FDH/styleganL/singles/5072/original.png}
\caption{Original}
\end{subfigure}%%
\begin{subfigure}[t]{0.125\textwidth}
\includegraphics[width=\textwidth]{appendix_figures/random_FDH/styleganL/singles/3219/masked_keypoints.png}
\includegraphics[width=\textwidth]{appendix_figures/random_FDH/styleganL/singles/3560/masked_keypoints.png}
\includegraphics[width=\textwidth]{appendix_figures/random_FDH/styleganL/singles/4420/masked_keypoints.png}
\includegraphics[width=\textwidth]{appendix_figures/random_FDH/styleganL/singles/4851/masked_keypoints.png}
\includegraphics[width=\textwidth]{appendix_figures/random_FDH/styleganL/singles/5072/masked_keypoints.png}
\caption{Condition}
\end{subfigure}%%
\begin{subfigure}[t]{0.125\textwidth}
\includegraphics[width=\textwidth]{appendix_figures/random_FDH/styleganL/singles/3219/fakes/0.png}
\includegraphics[width=\textwidth]{appendix_figures/random_FDH/styleganL/singles/3560/fakes/0.png}
\includegraphics[width=\textwidth]{appendix_figures/random_FDH/styleganL/singles/4420/fakes/0.png}
\includegraphics[width=\textwidth]{appendix_figures/random_FDH/styleganL/singles/4851/fakes/0.png}
\includegraphics[width=\textwidth]{appendix_figures/random_FDH/styleganL/singles/5072/fakes/0.png}
\caption{SG-GAN}
\end{subfigure}%%
\begin{subfigure}[t]{0.125\textwidth}
\includegraphics[width=\textwidth]{appendix_figures/random_FDH/styleganL/singles/3219/fakes/1.png}
\includegraphics[width=\textwidth]{appendix_figures/random_FDH/styleganL/singles/3560/fakes/1.png}
\includegraphics[width=\textwidth]{appendix_figures/random_FDH/styleganL/singles/4420/fakes/1.png}
\includegraphics[width=\textwidth]{appendix_figures/random_FDH/styleganL/singles/4851/fakes/1.png}
\includegraphics[width=\textwidth]{appendix_figures/random_FDH/styleganL/singles/5072/fakes/1.png}
\caption{SG-GAN}
\end{subfigure}%%
\begin{subfigure}[t]{0.125\textwidth}
\includegraphics[width=\textwidth]{appendix_figures/random_FDH/styleganL/singles/3219/fakes/2.png}
\includegraphics[width=\textwidth]{appendix_figures/random_FDH/styleganL/singles/3560/fakes/2.png}
\includegraphics[width=\textwidth]{appendix_figures/random_FDH/styleganL/singles/4420/fakes/2.png}
\includegraphics[width=\textwidth]{appendix_figures/random_FDH/styleganL/singles/4851/fakes/2.png}
\includegraphics[width=\textwidth]{appendix_figures/random_FDH/styleganL/singles/5072/fakes/2.png}
\caption{SG-GAN}
\end{subfigure}%%
\begin{subfigure}[t]{0.125\textwidth}
\includegraphics[width=\textwidth]{appendix_figures/random_FDH/im288/singles/3219/fakes/0.png}
\includegraphics[width=\textwidth]{appendix_figures/random_FDH/im288/singles/3560/fakes/0.png}
\includegraphics[width=\textwidth]{appendix_figures/random_FDH/im288/singles/4420/fakes/0.png}
\includegraphics[width=\textwidth]{appendix_figures/random_FDH/im288/singles/4851/fakes/0.png}
\includegraphics[width=\textwidth]{appendix_figures/random_FDH/im288/singles/5072/fakes/0.png}
\caption{\methodName}
\end{subfigure}%%
\begin{subfigure}[t]{0.125\textwidth}
\includegraphics[width=\textwidth]{appendix_figures/random_FDH/im288/singles/3219/fakes/1.png}
\includegraphics[width=\textwidth]{appendix_figures/random_FDH/im288/singles/3560/fakes/1.png}
\includegraphics[width=\textwidth]{appendix_figures/random_FDH/im288/singles/4420/fakes/1.png}
\includegraphics[width=\textwidth]{appendix_figures/random_FDH/im288/singles/4851/fakes/1.png}
\includegraphics[width=\textwidth]{appendix_figures/random_FDH/im288/singles/5072/fakes/1.png}
\caption{\methodName}
\end{subfigure}%%
\begin{subfigure}[t]{0.125\textwidth}
\includegraphics[width=\textwidth]{appendix_figures/random_FDH/im288/singles/3219/fakes/2.png}
\includegraphics[width=\textwidth]{appendix_figures/random_FDH/im288/singles/3560/fakes/2.png}
\includegraphics[width=\textwidth]{appendix_figures/random_FDH/im288/singles/4420/fakes/2.png}
\includegraphics[width=\textwidth]{appendix_figures/random_FDH/im288/singles/4851/fakes/2.png}
\includegraphics[width=\textwidth]{appendix_figures/random_FDH/im288/singles/5072/fakes/2.png}
\caption{\methodName}
\end{subfigure}%%
\caption{Random generated examples from FDH \cite{Hukkelas2022a} comparing \methodName to SG-GAN \cite{Hukkelas2022a}.
Note that all examples are generated with multi-modal truncation.
Surface map is not used by \methodName.}
\label{fig:fdh_random16}
\end{figure*}
\begin{figure*}[t]
\centering
\begin{subfigure}[t]{0.125\textwidth}
\includegraphics[width=\textwidth]{appendix_figures/random_FDH/styleganL/singles/6021/original.png}
\includegraphics[width=\textwidth]{appendix_figures/random_FDH/styleganL/singles/6036/original.png}
\includegraphics[width=\textwidth]{appendix_figures/random_FDH/styleganL/singles/6216/original.png}
\includegraphics[width=\textwidth]{appendix_figures/random_FDH/styleganL/singles/6744/original.png}
\includegraphics[width=\textwidth]{appendix_figures/random_FDH/styleganL/singles/6921/original.png}
\caption{Original}
\end{subfigure}%%
\begin{subfigure}[t]{0.125\textwidth}
\includegraphics[width=\textwidth]{appendix_figures/random_FDH/styleganL/singles/6021/masked_keypoints.png}
\includegraphics[width=\textwidth]{appendix_figures/random_FDH/styleganL/singles/6036/masked_keypoints.png}
\includegraphics[width=\textwidth]{appendix_figures/random_FDH/styleganL/singles/6216/masked_keypoints.png}
\includegraphics[width=\textwidth]{appendix_figures/random_FDH/styleganL/singles/6744/masked_keypoints.png}
\includegraphics[width=\textwidth]{appendix_figures/random_FDH/styleganL/singles/6921/masked_keypoints.png}
\caption{Condition}
\end{subfigure}%%
\begin{subfigure}[t]{0.125\textwidth}
\includegraphics[width=\textwidth]{appendix_figures/random_FDH/styleganL/singles/6021/fakes/0.png}
\includegraphics[width=\textwidth]{appendix_figures/random_FDH/styleganL/singles/6036/fakes/0.png}
\includegraphics[width=\textwidth]{appendix_figures/random_FDH/styleganL/singles/6216/fakes/0.png}
\includegraphics[width=\textwidth]{appendix_figures/random_FDH/styleganL/singles/6744/fakes/0.png}
\includegraphics[width=\textwidth]{appendix_figures/random_FDH/styleganL/singles/6921/fakes/0.png}
\caption{SG-GAN}
\end{subfigure}%%
\begin{subfigure}[t]{0.125\textwidth}
\includegraphics[width=\textwidth]{appendix_figures/random_FDH/styleganL/singles/6021/fakes/1.png}
\includegraphics[width=\textwidth]{appendix_figures/random_FDH/styleganL/singles/6036/fakes/1.png}
\includegraphics[width=\textwidth]{appendix_figures/random_FDH/styleganL/singles/6216/fakes/1.png}
\includegraphics[width=\textwidth]{appendix_figures/random_FDH/styleganL/singles/6744/fakes/1.png}
\includegraphics[width=\textwidth]{appendix_figures/random_FDH/styleganL/singles/6921/fakes/1.png}
\caption{SG-GAN}
\end{subfigure}%%
\begin{subfigure}[t]{0.125\textwidth}
\includegraphics[width=\textwidth]{appendix_figures/random_FDH/styleganL/singles/6021/fakes/2.png}
\includegraphics[width=\textwidth]{appendix_figures/random_FDH/styleganL/singles/6036/fakes/2.png}
\includegraphics[width=\textwidth]{appendix_figures/random_FDH/styleganL/singles/6216/fakes/2.png}
\includegraphics[width=\textwidth]{appendix_figures/random_FDH/styleganL/singles/6744/fakes/2.png}
\includegraphics[width=\textwidth]{appendix_figures/random_FDH/styleganL/singles/6921/fakes/2.png}
\caption{SG-GAN}
\end{subfigure}%%
\begin{subfigure}[t]{0.125\textwidth}
\includegraphics[width=\textwidth]{appendix_figures/random_FDH/im288/singles/6021/fakes/0.png}
\includegraphics[width=\textwidth]{appendix_figures/random_FDH/im288/singles/6036/fakes/0.png}
\includegraphics[width=\textwidth]{appendix_figures/random_FDH/im288/singles/6216/fakes/0.png}
\includegraphics[width=\textwidth]{appendix_figures/random_FDH/im288/singles/6744/fakes/0.png}
\includegraphics[width=\textwidth]{appendix_figures/random_FDH/im288/singles/6921/fakes/0.png}
\caption{\methodName}
\end{subfigure}%%
\begin{subfigure}[t]{0.125\textwidth}
\includegraphics[width=\textwidth]{appendix_figures/random_FDH/im288/singles/6021/fakes/1.png}
\includegraphics[width=\textwidth]{appendix_figures/random_FDH/im288/singles/6036/fakes/1.png}
\includegraphics[width=\textwidth]{appendix_figures/random_FDH/im288/singles/6216/fakes/1.png}
\includegraphics[width=\textwidth]{appendix_figures/random_FDH/im288/singles/6744/fakes/1.png}
\includegraphics[width=\textwidth]{appendix_figures/random_FDH/im288/singles/6921/fakes/1.png}
\caption{\methodName}
\end{subfigure}%%
\begin{subfigure}[t]{0.125\textwidth}
\includegraphics[width=\textwidth]{appendix_figures/random_FDH/im288/singles/6021/fakes/2.png}
\includegraphics[width=\textwidth]{appendix_figures/random_FDH/im288/singles/6036/fakes/2.png}
\includegraphics[width=\textwidth]{appendix_figures/random_FDH/im288/singles/6216/fakes/2.png}
\includegraphics[width=\textwidth]{appendix_figures/random_FDH/im288/singles/6744/fakes/2.png}
\includegraphics[width=\textwidth]{appendix_figures/random_FDH/im288/singles/6921/fakes/2.png}
\caption{\methodName}
\end{subfigure}%%
\caption{Random generated examples from FDH \cite{Hukkelas2022a} comparing \methodName to SG-GAN \cite{Hukkelas2022a}.
Note that all examples are generated with multi-modal truncation.
Surface map is not used by \methodName.}
\label{fig:fdh_random17}
\end{figure*}
\begin{figure*}[t]
\centering
\begin{subfigure}[t]{0.125\textwidth}
\includegraphics[width=\textwidth]{appendix_figures/random_FDH/styleganL/singles/7108/original.png}
\includegraphics[width=\textwidth]{appendix_figures/random_FDH/styleganL/singles/755/original.png}
\includegraphics[width=\textwidth]{appendix_figures/random_FDH/styleganL/singles/7599/original.png}
\includegraphics[width=\textwidth]{appendix_figures/random_FDH/styleganL/singles/7877/original.png}
\includegraphics[width=\textwidth]{appendix_figures/random_FDH/styleganL/singles/797/original.png}
\caption{Original}
\end{subfigure}%%
\begin{subfigure}[t]{0.125\textwidth}
\includegraphics[width=\textwidth]{appendix_figures/random_FDH/styleganL/singles/7108/masked_keypoints.png}
\includegraphics[width=\textwidth]{appendix_figures/random_FDH/styleganL/singles/755/masked_keypoints.png}
\includegraphics[width=\textwidth]{appendix_figures/random_FDH/styleganL/singles/7599/masked_keypoints.png}
\includegraphics[width=\textwidth]{appendix_figures/random_FDH/styleganL/singles/7877/masked_keypoints.png}
\includegraphics[width=\textwidth]{appendix_figures/random_FDH/styleganL/singles/797/masked_keypoints.png}
\caption{Condition}
\end{subfigure}%%
\begin{subfigure}[t]{0.125\textwidth}
\includegraphics[width=\textwidth]{appendix_figures/random_FDH/styleganL/singles/7108/fakes/0.png}
\includegraphics[width=\textwidth]{appendix_figures/random_FDH/styleganL/singles/755/fakes/0.png}
\includegraphics[width=\textwidth]{appendix_figures/random_FDH/styleganL/singles/7599/fakes/0.png}
\includegraphics[width=\textwidth]{appendix_figures/random_FDH/styleganL/singles/7877/fakes/0.png}
\includegraphics[width=\textwidth]{appendix_figures/random_FDH/styleganL/singles/797/fakes/0.png}
\caption{SG-GAN}
\end{subfigure}%%
\begin{subfigure}[t]{0.125\textwidth}
\includegraphics[width=\textwidth]{appendix_figures/random_FDH/styleganL/singles/7108/fakes/1.png}
\includegraphics[width=\textwidth]{appendix_figures/random_FDH/styleganL/singles/755/fakes/1.png}
\includegraphics[width=\textwidth]{appendix_figures/random_FDH/styleganL/singles/7599/fakes/1.png}
\includegraphics[width=\textwidth]{appendix_figures/random_FDH/styleganL/singles/7877/fakes/1.png}
\includegraphics[width=\textwidth]{appendix_figures/random_FDH/styleganL/singles/797/fakes/1.png}
\caption{SG-GAN}
\end{subfigure}%%
\begin{subfigure}[t]{0.125\textwidth}
\includegraphics[width=\textwidth]{appendix_figures/random_FDH/styleganL/singles/7108/fakes/2.png}
\includegraphics[width=\textwidth]{appendix_figures/random_FDH/styleganL/singles/755/fakes/2.png}
\includegraphics[width=\textwidth]{appendix_figures/random_FDH/styleganL/singles/7599/fakes/2.png}
\includegraphics[width=\textwidth]{appendix_figures/random_FDH/styleganL/singles/7877/fakes/2.png}
\includegraphics[width=\textwidth]{appendix_figures/random_FDH/styleganL/singles/797/fakes/2.png}
\caption{SG-GAN}
\end{subfigure}%%
\begin{subfigure}[t]{0.125\textwidth}
\includegraphics[width=\textwidth]{appendix_figures/random_FDH/im288/singles/7108/fakes/0.png}
\includegraphics[width=\textwidth]{appendix_figures/random_FDH/im288/singles/755/fakes/0.png}
\includegraphics[width=\textwidth]{appendix_figures/random_FDH/im288/singles/7599/fakes/0.png}
\includegraphics[width=\textwidth]{appendix_figures/random_FDH/im288/singles/7877/fakes/0.png}
\includegraphics[width=\textwidth]{appendix_figures/random_FDH/im288/singles/797/fakes/0.png}
\caption{\methodName}
\end{subfigure}%%
\begin{subfigure}[t]{0.125\textwidth}
\includegraphics[width=\textwidth]{appendix_figures/random_FDH/im288/singles/7108/fakes/1.png}
\includegraphics[width=\textwidth]{appendix_figures/random_FDH/im288/singles/755/fakes/1.png}
\includegraphics[width=\textwidth]{appendix_figures/random_FDH/im288/singles/7599/fakes/1.png}
\includegraphics[width=\textwidth]{appendix_figures/random_FDH/im288/singles/7877/fakes/1.png}
\includegraphics[width=\textwidth]{appendix_figures/random_FDH/im288/singles/797/fakes/1.png}
\caption{\methodName}
\end{subfigure}%%
\begin{subfigure}[t]{0.125\textwidth}
\includegraphics[width=\textwidth]{appendix_figures/random_FDH/im288/singles/7108/fakes/2.png}
\includegraphics[width=\textwidth]{appendix_figures/random_FDH/im288/singles/755/fakes/2.png}
\includegraphics[width=\textwidth]{appendix_figures/random_FDH/im288/singles/7599/fakes/2.png}
\includegraphics[width=\textwidth]{appendix_figures/random_FDH/im288/singles/7877/fakes/2.png}
\includegraphics[width=\textwidth]{appendix_figures/random_FDH/im288/singles/797/fakes/2.png}
\caption{\methodName}
\end{subfigure}%%
\caption{Random generated examples from FDH \cite{Hukkelas2022a} comparing \methodName to SG-GAN \cite{Hukkelas2022a}.
Note that all examples are generated with multi-modal truncation.
Surface map is not used by \methodName.}
\label{fig:fdh_random18}
\end{figure*}
\begin{figure*}[t]
\centering
\begin{subfigure}[t]{0.125\textwidth}
\includegraphics[width=\textwidth]{appendix_figures/random_FDH/styleganL/singles/8622/original.png}
\includegraphics[width=\textwidth]{appendix_figures/random_FDH/styleganL/singles/8736/original.png}
\includegraphics[width=\textwidth]{appendix_figures/random_FDH/styleganL/singles/9225/original.png}
\includegraphics[width=\textwidth]{appendix_figures/random_FDH/styleganL/singles/9781/original.png}
\includegraphics[width=\textwidth]{appendix_figures/random_FDH/styleganL/singles/9845/original.png}
\caption{Original}
\end{subfigure}%%
\begin{subfigure}[t]{0.125\textwidth}
\includegraphics[width=\textwidth]{appendix_figures/random_FDH/styleganL/singles/8622/masked_keypoints.png}
\includegraphics[width=\textwidth]{appendix_figures/random_FDH/styleganL/singles/8736/masked_keypoints.png}
\includegraphics[width=\textwidth]{appendix_figures/random_FDH/styleganL/singles/9225/masked_keypoints.png}
\includegraphics[width=\textwidth]{appendix_figures/random_FDH/styleganL/singles/9781/masked_keypoints.png}
\includegraphics[width=\textwidth]{appendix_figures/random_FDH/styleganL/singles/9845/masked_keypoints.png}
\caption{Condition}
\end{subfigure}%%
\begin{subfigure}[t]{0.125\textwidth}
\includegraphics[width=\textwidth]{appendix_figures/random_FDH/styleganL/singles/8622/fakes/0.png}
\includegraphics[width=\textwidth]{appendix_figures/random_FDH/styleganL/singles/8736/fakes/0.png}
\includegraphics[width=\textwidth]{appendix_figures/random_FDH/styleganL/singles/9225/fakes/0.png}
\includegraphics[width=\textwidth]{appendix_figures/random_FDH/styleganL/singles/9781/fakes/0.png}
\includegraphics[width=\textwidth]{appendix_figures/random_FDH/styleganL/singles/9845/fakes/0.png}
\caption{SG-GAN}
\end{subfigure}%%
\begin{subfigure}[t]{0.125\textwidth}
\includegraphics[width=\textwidth]{appendix_figures/random_FDH/styleganL/singles/8622/fakes/1.png}
\includegraphics[width=\textwidth]{appendix_figures/random_FDH/styleganL/singles/8736/fakes/1.png}
\includegraphics[width=\textwidth]{appendix_figures/random_FDH/styleganL/singles/9225/fakes/1.png}
\includegraphics[width=\textwidth]{appendix_figures/random_FDH/styleganL/singles/9781/fakes/1.png}
\includegraphics[width=\textwidth]{appendix_figures/random_FDH/styleganL/singles/9845/fakes/1.png}
\caption{SG-GAN}
\end{subfigure}%%
\begin{subfigure}[t]{0.125\textwidth}
\includegraphics[width=\textwidth]{appendix_figures/random_FDH/styleganL/singles/8622/fakes/2.png}
\includegraphics[width=\textwidth]{appendix_figures/random_FDH/styleganL/singles/8736/fakes/2.png}
\includegraphics[width=\textwidth]{appendix_figures/random_FDH/styleganL/singles/9225/fakes/2.png}
\includegraphics[width=\textwidth]{appendix_figures/random_FDH/styleganL/singles/9781/fakes/2.png}
\includegraphics[width=\textwidth]{appendix_figures/random_FDH/styleganL/singles/9845/fakes/2.png}
\caption{SG-GAN}
\end{subfigure}%%
\begin{subfigure}[t]{0.125\textwidth}
\includegraphics[width=\textwidth]{appendix_figures/random_FDH/im288/singles/8622/fakes/0.png}
\includegraphics[width=\textwidth]{appendix_figures/random_FDH/im288/singles/8736/fakes/0.png}
\includegraphics[width=\textwidth]{appendix_figures/random_FDH/im288/singles/9225/fakes/0.png}
\includegraphics[width=\textwidth]{appendix_figures/random_FDH/im288/singles/9781/fakes/0.png}
\includegraphics[width=\textwidth]{appendix_figures/random_FDH/im288/singles/9845/fakes/0.png}
\caption{\methodName}
\end{subfigure}%%
\begin{subfigure}[t]{0.125\textwidth}
\includegraphics[width=\textwidth]{appendix_figures/random_FDH/im288/singles/8622/fakes/1.png}
\includegraphics[width=\textwidth]{appendix_figures/random_FDH/im288/singles/8736/fakes/1.png}
\includegraphics[width=\textwidth]{appendix_figures/random_FDH/im288/singles/9225/fakes/1.png}
\includegraphics[width=\textwidth]{appendix_figures/random_FDH/im288/singles/9781/fakes/1.png}
\includegraphics[width=\textwidth]{appendix_figures/random_FDH/im288/singles/9845/fakes/1.png}
\caption{\methodName}
\end{subfigure}%%
\begin{subfigure}[t]{0.125\textwidth}
\includegraphics[width=\textwidth]{appendix_figures/random_FDH/im288/singles/8622/fakes/2.png}
\includegraphics[width=\textwidth]{appendix_figures/random_FDH/im288/singles/8736/fakes/2.png}
\includegraphics[width=\textwidth]{appendix_figures/random_FDH/im288/singles/9225/fakes/2.png}
\includegraphics[width=\textwidth]{appendix_figures/random_FDH/im288/singles/9781/fakes/2.png}
\includegraphics[width=\textwidth]{appendix_figures/random_FDH/im288/singles/9845/fakes/2.png}
\caption{\methodName}
\end{subfigure}%%
\caption{Random generated examples from FDH \cite{Hukkelas2022a} comparing \methodName to SG-GAN \cite{Hukkelas2022a}.
Note that all examples are generated with multi-modal truncation.
Surface map is not used by \methodName.}
\label{fig:fdh_random19}
\end{figure*}

\section{\methodName \vs SG-GANs for Anonymization}
We have integrated \methodName in DeepPrivacy2 \cite{Hukkelas2022a} to support anonymization.
\Cref{fig:comparison_to_SGGAN_anonymization} compares \methodName to Surface-Guided GANs \cite{Hukkelas2022} (DeepPrivacy2 variant \cite{Hukkelas2022a}).
Note that the majority of pedestrians are not anonymized by SG-GAN, as DensePose fails to detect pedestrians further away from the camera.
In addition, we note that the synthesis quality of \methodName is notably better for all pedestrians in the scene.

\begin{figure*}
    \centering
    \begin{subfigure}{.8\textwidth}
        \includegraphics[width=\textwidth]{figures/anonymization_comparison/strasbourg_000000_015764_leftImg8bit.jpg}
        \caption{Original Image}
    \end{subfigure}
    \begin{subfigure}{.8\textwidth}
        \includegraphics[width=\textwidth]{figures/anonymization_comparison/strasbourg_000000_015764_leftImg8bit_SGGAN.png}
        \caption{Anonymized with DeepPrivacy2 \cite{Hukkelas2022a}}
    \end{subfigure}
    \begin{subfigure}{.8\textwidth}
        \includegraphics[width=\textwidth]{figures/anonymization_comparison/strasbourg_000000_015764_leftImg8bit_TriAGAN.jpg}
        \caption{Anonymized with \methodName}
    \end{subfigure}
    \caption{Comparison of anonymization with \methodName \vs SG-GAN \cite{Hukkelas2022} trained following DeepPrivacy2 \cite{Hukkelas2022a}.}
    \label{fig:comparison_to_SGGAN_anonymization}
\end{figure*}
