# Supplementary material for: Synthesizing Anyone, Anywhere, in Any Pose
Source: arXiv:2304.03164 source file (2023-11-05)
Supplement: Supplementary file 2 [file grid0.tex]

\begin{figure*}[t]
\centering
\begin{subfigure}[t]{0.125\textwidth}
\includegraphics[width=\textwidth]{appendix_figures/random_FDH/styleganL/singles/10200/original.png}
\includegraphics[width=\textwidth]{appendix_figures/random_FDH/styleganL/singles/10327/original.png}
\includegraphics[width=\textwidth]{appendix_figures/random_FDH/styleganL/singles/10368/original.png}
\includegraphics[width=\textwidth]{appendix_figures/random_FDH/styleganL/singles/10799/original.png}
\includegraphics[width=\textwidth]{appendix_figures/random_FDH/styleganL/singles/11122/original.png}
\caption{Original}
\end{subfigure}%%
\begin{subfigure}[t]{0.125\textwidth}
\includegraphics[width=\textwidth]{appendix_figures/random_FDH/styleganL/singles/10200/masked_keypoints.png}
\includegraphics[width=\textwidth]{appendix_figures/random_FDH/styleganL/singles/10327/masked_keypoints.png}
\includegraphics[width=\textwidth]{appendix_figures/random_FDH/styleganL/singles/10368/masked_keypoints.png}
\includegraphics[width=\textwidth]{appendix_figures/random_FDH/styleganL/singles/10799/masked_keypoints.png}
\includegraphics[width=\textwidth]{appendix_figures/random_FDH/styleganL/singles/11122/masked_keypoints.png}
\caption{Condition}
\end{subfigure}%%
\begin{subfigure}[t]{0.125\textwidth}
\includegraphics[width=\textwidth]{appendix_figures/random_FDH/styleganL/singles/10200/fakes/0.png}
\includegraphics[width=\textwidth]{appendix_figures/random_FDH/styleganL/singles/10327/fakes/0.png}
\includegraphics[width=\textwidth]{appendix_figures/random_FDH/styleganL/singles/10368/fakes/0.png}
\includegraphics[width=\textwidth]{appendix_figures/random_FDH/styleganL/singles/10799/fakes/0.png}
\includegraphics[width=\textwidth]{appendix_figures/random_FDH/styleganL/singles/11122/fakes/0.png}
\caption{SG-GAN}
\end{subfigure}%%
\begin{subfigure}[t]{0.125\textwidth}
\includegraphics[width=\textwidth]{appendix_figures/random_FDH/styleganL/singles/10200/fakes/1.png}
\includegraphics[width=\textwidth]{appendix_figures/random_FDH/styleganL/singles/10327/fakes/1.png}
\includegraphics[width=\textwidth]{appendix_figures/random_FDH/styleganL/singles/10368/fakes/1.png}
\includegraphics[width=\textwidth]{appendix_figures/random_FDH/styleganL/singles/10799/fakes/1.png}
\includegraphics[width=\textwidth]{appendix_figures/random_FDH/styleganL/singles/11122/fakes/1.png}
\caption{SG-GAN}
\end{subfigure}%%
\begin{subfigure}[t]{0.125\textwidth}
\includegraphics[width=\textwidth]{appendix_figures/random_FDH/styleganL/singles/10200/fakes/2.png}
\includegraphics[width=\textwidth]{appendix_figures/random_FDH/styleganL/singles/10327/fakes/2.png}
\includegraphics[width=\textwidth]{appendix_figures/random_FDH/styleganL/singles/10368/fakes/2.png}
\includegraphics[width=\textwidth]{appendix_figures/random_FDH/styleganL/singles/10799/fakes/2.png}
\includegraphics[width=\textwidth]{appendix_figures/random_FDH/styleganL/singles/11122/fakes/2.png}
\caption{SG-GAN}
\end{subfigure}%%
\begin{subfigure}[t]{0.125\textwidth}
\includegraphics[width=\textwidth]{appendix_figures/random_FDH/im288/singles/10200/fakes/0.png}
\includegraphics[width=\textwidth]{appendix_figures/random_FDH/im288/singles/10327/fakes/0.png}
\includegraphics[width=\textwidth]{appendix_figures/random_FDH/im288/singles/10368/fakes/0.png}
\includegraphics[width=\textwidth]{appendix_figures/random_FDH/im288/singles/10799/fakes/0.png}
\includegraphics[width=\textwidth]{appendix_figures/random_FDH/im288/singles/11122/fakes/0.png}
\caption{\methodName}
\end{subfigure}%%
\begin{subfigure}[t]{0.125\textwidth}
\includegraphics[width=\textwidth]{appendix_figures/random_FDH/im288/singles/10200/fakes/1.png}
\includegraphics[width=\textwidth]{appendix_figures/random_FDH/im288/singles/10327/fakes/1.png}
\includegraphics[width=\textwidth]{appendix_figures/random_FDH/im288/singles/10368/fakes/1.png}
\includegraphics[width=\textwidth]{appendix_figures/random_FDH/im288/singles/10799/fakes/1.png}
\includegraphics[width=\textwidth]{appendix_figures/random_FDH/im288/singles/11122/fakes/1.png}
\caption{\methodName}
\end{subfigure}%%
\begin{subfigure}[t]{0.125\textwidth}
\includegraphics[width=\textwidth]{appendix_figures/random_FDH/im288/singles/10200/fakes/2.png}
\includegraphics[width=\textwidth]{appendix_figures/random_FDH/im288/singles/10327/fakes/2.png}
\includegraphics[width=\textwidth]{appendix_figures/random_FDH/im288/singles/10368/fakes/2.png}
\includegraphics[width=\textwidth]{appendix_figures/random_FDH/im288/singles/10799/fakes/2.png}
\includegraphics[width=\textwidth]{appendix_figures/random_FDH/im288/singles/11122/fakes/2.png}
\caption{\methodName}
\end{subfigure}%%
\caption{Random generated examples from FDH \cite{Hukkelas2022a} comparing \methodName to SG-GAN \cite{Hukkelas2022a}.
Note that all examples are generated with multi-modal truncation.
Surface map is not used by \methodName.}
\label{fig:fdh_random0}
\end{figure*}
