# Supplementary material for: Synthesizing Anyone, Anywhere, in Any Pose
Source: arXiv:2304.03164 source file (2023-11-05)
Supplement: Supplementary file 12 [file grid18.tex]

\begin{figure*}[t]
\centering
\begin{subfigure}[t]{0.125\textwidth}
\includegraphics[width=\textwidth]{appendix_figures/random_FDH/styleganL/singles/7108/original.png}
\includegraphics[width=\textwidth]{appendix_figures/random_FDH/styleganL/singles/755/original.png}
\includegraphics[width=\textwidth]{appendix_figures/random_FDH/styleganL/singles/7599/original.png}
\includegraphics[width=\textwidth]{appendix_figures/random_FDH/styleganL/singles/7877/original.png}
\includegraphics[width=\textwidth]{appendix_figures/random_FDH/styleganL/singles/797/original.png}
\caption{Original}
\end{subfigure}%%
\begin{subfigure}[t]{0.125\textwidth}
\includegraphics[width=\textwidth]{appendix_figures/random_FDH/styleganL/singles/7108/masked_keypoints.png}
\includegraphics[width=\textwidth]{appendix_figures/random_FDH/styleganL/singles/755/masked_keypoints.png}
\includegraphics[width=\textwidth]{appendix_figures/random_FDH/styleganL/singles/7599/masked_keypoints.png}
\includegraphics[width=\textwidth]{appendix_figures/random_FDH/styleganL/singles/7877/masked_keypoints.png}
\includegraphics[width=\textwidth]{appendix_figures/random_FDH/styleganL/singles/797/masked_keypoints.png}
\caption{Condition}
\end{subfigure}%%
\begin{subfigure}[t]{0.125\textwidth}
\includegraphics[width=\textwidth]{appendix_figures/random_FDH/styleganL/singles/7108/fakes/0.png}
\includegraphics[width=\textwidth]{appendix_figures/random_FDH/styleganL/singles/755/fakes/0.png}
\includegraphics[width=\textwidth]{appendix_figures/random_FDH/styleganL/singles/7599/fakes/0.png}
\includegraphics[width=\textwidth]{appendix_figures/random_FDH/styleganL/singles/7877/fakes/0.png}
\includegraphics[width=\textwidth]{appendix_figures/random_FDH/styleganL/singles/797/fakes/0.png}
\caption{SG-GAN}
\end{subfigure}%%
\begin{subfigure}[t]{0.125\textwidth}
\includegraphics[width=\textwidth]{appendix_figures/random_FDH/styleganL/singles/7108/fakes/1.png}
\includegraphics[width=\textwidth]{appendix_figures/random_FDH/styleganL/singles/755/fakes/1.png}
\includegraphics[width=\textwidth]{appendix_figures/random_FDH/styleganL/singles/7599/fakes/1.png}
\includegraphics[width=\textwidth]{appendix_figures/random_FDH/styleganL/singles/7877/fakes/1.png}
\includegraphics[width=\textwidth]{appendix_figures/random_FDH/styleganL/singles/797/fakes/1.png}
\caption{SG-GAN}
\end{subfigure}%%
\begin{subfigure}[t]{0.125\textwidth}
\includegraphics[width=\textwidth]{appendix_figures/random_FDH/styleganL/singles/7108/fakes/2.png}
\includegraphics[width=\textwidth]{appendix_figures/random_FDH/styleganL/singles/755/fakes/2.png}
\includegraphics[width=\textwidth]{appendix_figures/random_FDH/styleganL/singles/7599/fakes/2.png}
\includegraphics[width=\textwidth]{appendix_figures/random_FDH/styleganL/singles/7877/fakes/2.png}
\includegraphics[width=\textwidth]{appendix_figures/random_FDH/styleganL/singles/797/fakes/2.png}
\caption{SG-GAN}
\end{subfigure}%%
\begin{subfigure}[t]{0.125\textwidth}
\includegraphics[width=\textwidth]{appendix_figures/random_FDH/im288/singles/7108/fakes/0.png}
\includegraphics[width=\textwidth]{appendix_figures/random_FDH/im288/singles/755/fakes/0.png}
\includegraphics[width=\textwidth]{appendix_figures/random_FDH/im288/singles/7599/fakes/0.png}
\includegraphics[width=\textwidth]{appendix_figures/random_FDH/im288/singles/7877/fakes/0.png}
\includegraphics[width=\textwidth]{appendix_figures/random_FDH/im288/singles/797/fakes/0.png}
\caption{\methodName}
\end{subfigure}%%
\begin{subfigure}[t]{0.125\textwidth}
\includegraphics[width=\textwidth]{appendix_figures/random_FDH/im288/singles/7108/fakes/1.png}
\includegraphics[width=\textwidth]{appendix_figures/random_FDH/im288/singles/755/fakes/1.png}
\includegraphics[width=\textwidth]{appendix_figures/random_FDH/im288/singles/7599/fakes/1.png}
\includegraphics[width=\textwidth]{appendix_figures/random_FDH/im288/singles/7877/fakes/1.png}
\includegraphics[width=\textwidth]{appendix_figures/random_FDH/im288/singles/797/fakes/1.png}
\caption{\methodName}
\end{subfigure}%%
\begin{subfigure}[t]{0.125\textwidth}
\includegraphics[width=\textwidth]{appendix_figures/random_FDH/im288/singles/7108/fakes/2.png}
\includegraphics[width=\textwidth]{appendix_figures/random_FDH/im288/singles/755/fakes/2.png}
\includegraphics[width=\textwidth]{appendix_figures/random_FDH/im288/singles/7599/fakes/2.png}
\includegraphics[width=\textwidth]{appendix_figures/random_FDH/im288/singles/7877/fakes/2.png}
\includegraphics[width=\textwidth]{appendix_figures/random_FDH/im288/singles/797/fakes/2.png}
\caption{\methodName}
\end{subfigure}%%
\caption{Random generated examples from FDH \cite{Hukkelas2022a} comparing \methodName to SG-GAN \cite{Hukkelas2022a}.
Note that all examples are generated with multi-modal truncation.
Surface map is not used by \methodName.}
\label{fig:fdh_random18}
\end{figure*}
