# Supplementary material for: Synthesizing Anyone, Anywhere, in Any Pose
Source: arXiv:2304.03164 source file (2023-11-05)
Supplement: Supplementary file 15 [file grid3.tex]

\begin{figure*}[t]
\centering
\begin{subfigure}[t]{0.125\textwidth}
\includegraphics[width=\textwidth]{appendix_figures/random_FDH/styleganL/singles/14879/original.png}
\includegraphics[width=\textwidth]{appendix_figures/random_FDH/styleganL/singles/14935/original.png}
\includegraphics[width=\textwidth]{appendix_figures/random_FDH/styleganL/singles/15115/original.png}
\includegraphics[width=\textwidth]{appendix_figures/random_FDH/styleganL/singles/15186/original.png}
\includegraphics[width=\textwidth]{appendix_figures/random_FDH/styleganL/singles/15246/original.png}
\caption{Original}
\end{subfigure}%%
\begin{subfigure}[t]{0.125\textwidth}
\includegraphics[width=\textwidth]{appendix_figures/random_FDH/styleganL/singles/14879/masked_keypoints.png}
\includegraphics[width=\textwidth]{appendix_figures/random_FDH/styleganL/singles/14935/masked_keypoints.png}
\includegraphics[width=\textwidth]{appendix_figures/random_FDH/styleganL/singles/15115/masked_keypoints.png}
\includegraphics[width=\textwidth]{appendix_figures/random_FDH/styleganL/singles/15186/masked_keypoints.png}
\includegraphics[width=\textwidth]{appendix_figures/random_FDH/styleganL/singles/15246/masked_keypoints.png}
\caption{Condition}
\end{subfigure}%%
\begin{subfigure}[t]{0.125\textwidth}
\includegraphics[width=\textwidth]{appendix_figures/random_FDH/styleganL/singles/14879/fakes/0.png}
\includegraphics[width=\textwidth]{appendix_figures/random_FDH/styleganL/singles/14935/fakes/0.png}
\includegraphics[width=\textwidth]{appendix_figures/random_FDH/styleganL/singles/15115/fakes/0.png}
\includegraphics[width=\textwidth]{appendix_figures/random_FDH/styleganL/singles/15186/fakes/0.png}
\includegraphics[width=\textwidth]{appendix_figures/random_FDH/styleganL/singles/15246/fakes/0.png}
\caption{SG-GAN}
\end{subfigure}%%
\begin{subfigure}[t]{0.125\textwidth}
\includegraphics[width=\textwidth]{appendix_figures/random_FDH/styleganL/singles/14879/fakes/1.png}
\includegraphics[width=\textwidth]{appendix_figures/random_FDH/styleganL/singles/14935/fakes/1.png}
\includegraphics[width=\textwidth]{appendix_figures/random_FDH/styleganL/singles/15115/fakes/1.png}
\includegraphics[width=\textwidth]{appendix_figures/random_FDH/styleganL/singles/15186/fakes/1.png}
\includegraphics[width=\textwidth]{appendix_figures/random_FDH/styleganL/singles/15246/fakes/1.png}
\caption{SG-GAN}
\end{subfigure}%%
\begin{subfigure}[t]{0.125\textwidth}
\includegraphics[width=\textwidth]{appendix_figures/random_FDH/styleganL/singles/14879/fakes/2.png}
\includegraphics[width=\textwidth]{appendix_figures/random_FDH/styleganL/singles/14935/fakes/2.png}
\includegraphics[width=\textwidth]{appendix_figures/random_FDH/styleganL/singles/15115/fakes/2.png}
\includegraphics[width=\textwidth]{appendix_figures/random_FDH/styleganL/singles/15186/fakes/2.png}
\includegraphics[width=\textwidth]{appendix_figures/random_FDH/styleganL/singles/15246/fakes/2.png}
\caption{SG-GAN}
\end{subfigure}%%
\begin{subfigure}[t]{0.125\textwidth}
\includegraphics[width=\textwidth]{appendix_figures/random_FDH/im288/singles/14879/fakes/0.png}
\includegraphics[width=\textwidth]{appendix_figures/random_FDH/im288/singles/14935/fakes/0.png}
\includegraphics[width=\textwidth]{appendix_figures/random_FDH/im288/singles/15115/fakes/0.png}
\includegraphics[width=\textwidth]{appendix_figures/random_FDH/im288/singles/15186/fakes/0.png}
\includegraphics[width=\textwidth]{appendix_figures/random_FDH/im288/singles/15246/fakes/0.png}
\caption{\methodName}
\end{subfigure}%%
\begin{subfigure}[t]{0.125\textwidth}
\includegraphics[width=\textwidth]{appendix_figures/random_FDH/im288/singles/14879/fakes/1.png}
\includegraphics[width=\textwidth]{appendix_figures/random_FDH/im288/singles/14935/fakes/1.png}
\includegraphics[width=\textwidth]{appendix_figures/random_FDH/im288/singles/15115/fakes/1.png}
\includegraphics[width=\textwidth]{appendix_figures/random_FDH/im288/singles/15186/fakes/1.png}
\includegraphics[width=\textwidth]{appendix_figures/random_FDH/im288/singles/15246/fakes/1.png}
\caption{\methodName}
\end{subfigure}%%
\begin{subfigure}[t]{0.125\textwidth}
\includegraphics[width=\textwidth]{appendix_figures/random_FDH/im288/singles/14879/fakes/2.png}
\includegraphics[width=\textwidth]{appendix_figures/random_FDH/im288/singles/14935/fakes/2.png}
\includegraphics[width=\textwidth]{appendix_figures/random_FDH/im288/singles/15115/fakes/2.png}
\includegraphics[width=\textwidth]{appendix_figures/random_FDH/im288/singles/15186/fakes/2.png}
\includegraphics[width=\textwidth]{appendix_figures/random_FDH/im288/singles/15246/fakes/2.png}
\caption{\methodName}
\end{subfigure}%%
\caption{Random generated examples from FDH \cite{Hukkelas2022a} comparing \methodName to SG-GAN \cite{Hukkelas2022a}.
Note that all examples are generated with multi-modal truncation.
Surface map is not used by \methodName.}
\label{fig:fdh_random3}
\end{figure*}
